# Supplementary material for: Hypergraph Partitioning With Embeddings
Source: arXiv:1909.04016 source file (2020-08-25)
Supplement: Supplementary file 1 [file appendix.tex]

\begin{landscape}
  \section{Benchmark Graphs Details Plot}
  \label{sec:graph_plot}
  \begin{figure}[b]
    \centering
    \includegraphics[width=.95\linewidth, height=.85\textheight, keepaspectratio]{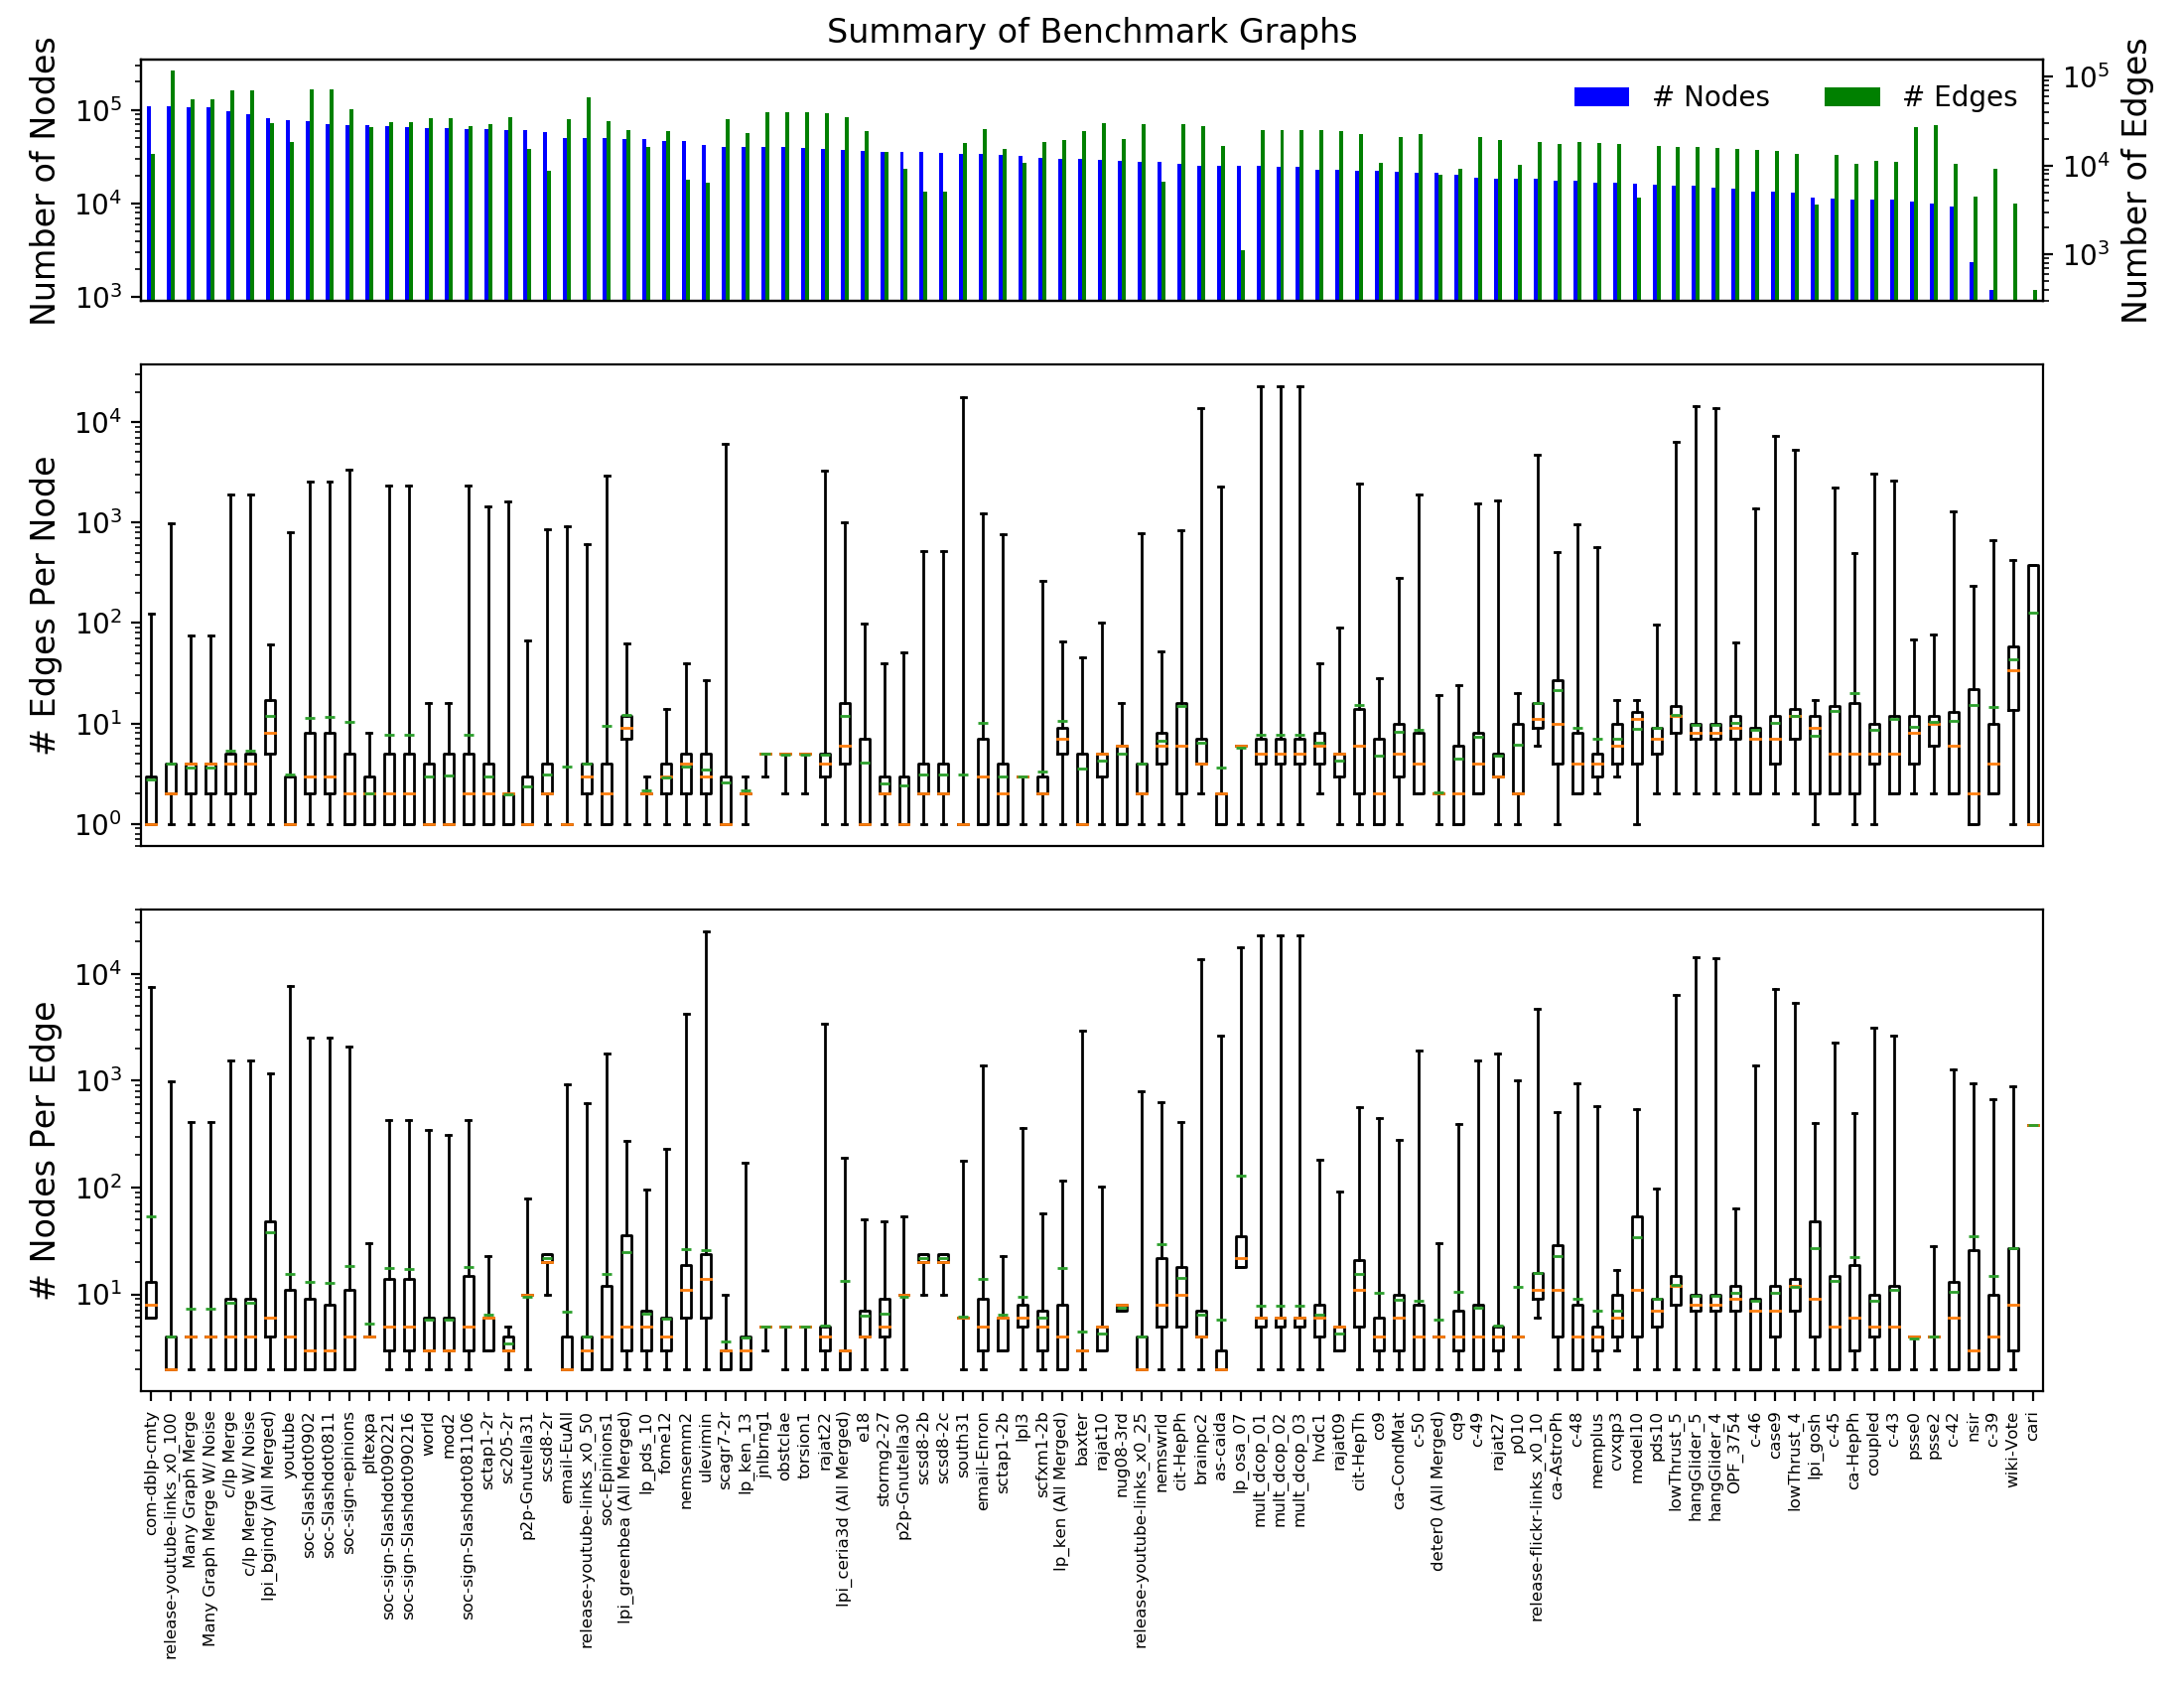}
    \caption{
      Distribution of nodes and edges for each hypergraph present in our
      benchmark. Graphs are sorted by number of nodes.
    }
    \label{fig:hypergraph_data}
  \end{figure}
\end{landscape}

\pagebreak
\section{Benchmark Graphs Details Table}
\label{sec:graph_table}
\begin{small}
\begin{longtable}{*{9}{l}}
\multirow{2}{*}{Hypergraph}
& \multirow{2}{*}{\# Node}
& \multirow{2}{*}{\# Edge}
& \multicolumn{3}{c}{Node Degree}
& \multicolumn{3}{c}{Edge Degree} \\
& &
& Med. & Mean & Std.
& Med. & Mean & Std. \\
\hline
\endhead
com-dblp-cmty&260998&13477&1&2.758&4.340&8&53.411&4.340 \\
release-youtube-links\_x0\_100&115782&115778&2&3.999&7.222&2&3.999&7.222 \\
Many Graph Mixture&110703&55307&4&3.645&2.970&4&7.296&2.970 \\
Many Graph Mixture W/ Noise&110703&55507&4&3.650&2.971&4&7.279&2.971 \\
c/lp Mixture&107776&69368&4&5.374&12.552&4&8.350&12.552 \\
c/lp Mixture W/ Noise&107776&69568&4&5.379&12.552&4&8.333&12.552 \\
lpi\_bgindy Mixture&97920&30322&8&11.824&9.319&6&38.182&9.319 \\
youtube&90581&18173&1&3.107&8.121&4&15.487&8.121 \\
soc-Slashdot0902&82159&71882&3&11.464&37.486&3&13.103&37.486 \\
soc-Slashdot0811&77355&70893&3&11.622&37.228&3&12.682&37.228 \\
soc-sign-epinions&76359&42470&2&10.327&43.547&4&18.567&43.547 \\
pltexpa&70364&26894&2&2.033&1.288&4&5.319&1.288 \\
soc-sign-Slashdot090221&69038&30670&2&7.761&33.115&5&17.471&33.115 \\
soc-sign-Slashdot090216&68836&30554&2&7.734&32.971&5&17.423&32.971 \\
world&66747&34106&1&2.974&2.751&3&5.820&2.751 \\
mod2&65990&34355&1&3.022&2.883&3&5.804&2.883 \\
soc-sign-Slashdot081106&64371&27753&2&7.783&32.163&5&18.051&32.163 \\
sctap1-2r&63426&28830&2&2.938&23.857&6&6.464&23.857 \\
sc205-2r&62422&35212&2&1.974&18.129&3&3.500&18.129 \\
p2p-Gnutella31&62023&15383&1&2.368&2.669&10&9.549&2.669 \\
scsd8-2r&60550&8650&2&3.141&22.885&20&21.990&22.885 \\
email-EuAll&60532&33292&1&3.765&24.650&2&6.846&24.650 \\
release-youtube-links\_x0\_50&57891&57888&3&3.999&7.222&3&3.999&7.222 \\
soc-Epinions1&50328&31149&2&9.530&39.646&4&15.398&39.646 \\
lpi\_greenbea Mixture&50319&24711&9&12.288&9.328&5&25.023&9.328 \\
lp\_pds\_10&49932&16239&2&2.149&0.424&5&6.607&0.424 \\
fome12&48920&24284&3&2.913&1.303&4&5.869&1.303 \\
nemsemm2&48857&6922&4&3.725&2.568&11&26.292&2.568 \\
ulevimin&46754&6394&3&3.515&2.714&14&25.703&2.714 \\
scagr7-2r&46679&32846&1&2.574&35.334&3&3.658&35.334 \\
lp\_ken\_13&42659&23393&2&2.157&0.542&3&3.933&0.542 \\
jnlbrng1&40000&40000&5&4.980&0.141&5&4.980&0.141 \\
obstclae&39996&39996&5&4.941&0.418&5&4.941&0.418 \\
torsion1&39996&39996&5&4.941&0.418&5&4.941&0.418 \\
rajat22&39801&38431&4&4.919&24.574&4&5.095&24.574 \\
lpi\_ceria3d Mixture&39600&35384&6&11.891&23.733&3&13.308&23.733 \\
e18&38601&24617&1&4.053&5.472&4&6.356&5.472 \\
stormg2-27&37485&14306&2&2.513&2.000&5&6.584&2.000 \\
p2p-Gnutella30&36345&9205&1&2.416&2.594&10&9.539&2.594 \\
scsd8-2b&35910&5130&2&3.140&17.607&20&21.982&17.607 \\
scsd8-2c&35910&5130&2&3.140&17.607&20&21.982&17.607 \\
south31&35885&17989&1&3.120&132.364&6&6.224&132.364 \\
email-Enron&35153&25481&3&10.140&33.809&5&13.989&33.809 \\
sctap1-2b&33858&15390&2&2.937&17.447&6&6.462&17.447 \\
lpl3&33686&10655&3&2.979&0.184&6&9.418&0.184 \\
scfxm1-2b&33047&18266&2&3.337&6.509&5&6.038&6.509 \\
lp\_ken Mixture&32418&19219&7&10.513&10.796&4&17.733&10.796 \\
baxter&30722&24255&1&3.528&5.359&3&4.469&5.359 \\
rajat10&30202&30101&5&4.311&1.116&5&4.326&1.116 \\
nug08-3rd&29856&19728&6&4.971&3.505&8&7.523&3.505 \\
release-youtube-links\_x0\_25&28945&28938&2&3.996&7.784&2&3.997&7.784 \\
nemswrld&28496&6512&6&6.743&5.108&8&29.507&5.108 \\
cit-HepPh&28093&29526&6&14.913&27.227&10&14.189&27.227 \\
brainpc2&27606&27606&4&6.498&131.257&4&6.498&131.257 \\
as-caida&26475&16538&2&3.657&29.016&2&5.855&29.016 \\
lp\_osa\_07&25067&1118&6&5.777&1.032&22&129.528&1.032 \\
mult\_dcop\_01&25019&24817&5&7.710&144.682&6&7.773&144.682 \\
mult\_dcop\_02&25019&24817&5&7.710&144.682&6&7.773&144.682 \\
mult\_dcop\_03&25019&24817&5&7.708&144.682&6&7.771&144.682 \\
hvdc1&24842&24842&6&6.440&2.936&6&6.440&2.936 \\
rajat09&24482&24391&5&4.309&1.117&5&4.325&1.117 \\
cit-HepTh&22908&22610&6&15.294&43.314&11&15.496&43.314 \\
co9&22829&10694&2&4.799&5.264&4&10.245&5.264 \\
ca-CondMat&22523&20760&5&8.194&10.671&6&8.890&10.671 \\
c-50&22401&22401&4&8.644&22.902&4&8.644&22.902 \\
deter0 Mixture&21872&7845&2&2.061&0.900&4&5.746&0.900 \\
cq9&21503&9247&2&4.493&4.673&4&10.449&4.673 \\
c-49&21132&21132&4&7.431&14.452&4&7.431&14.452 \\
rajat27&20540&19163&3&4.786&16.261&4&5.130&16.261 \\
p010&19081&10071&2&6.183&4.984&4&11.715&4.984 \\
release-flickr-links\_x0\_10&18612&18612&11&15.842&38.179&11&15.842&38.179 \\
ca-AstroPh&18479&17490&10&21.369&30.683&11&22.577&30.683 \\
c-48&18354&18354&4&9.049&16.866&4&9.049&16.866 \\
memplus&17758&17758&4&7.104&22.035&4&7.104&22.035 \\
cvxqp3&17500&17500&6&6.998&3.626&6&6.998&3.626 \\
model10&16819&4398&11&8.940&4.645&11&34.191&4.645 \\
pds10&16558&16558&7&9.038&7.258&7&9.038&7.258 \\
lowThrust\_5&16262&16262&12&12.198&70.124&12&12.198&70.124 \\
hangGlider\_5&16011&16011&8&9.696&112.427&8&9.696&112.427 \\
hangGlider\_4&15561&15561&8&9.609&110.835&8&9.609&110.835 \\
OPF\_3754&15435&15435&9&10.254&5.531&9&10.254&5.531 \\
c-46&14913&14913&7&8.744&42.022&7&8.744&42.022 \\
case9&14453&14453&7&10.238&105.257&7&10.238&105.257 \\
lowThrust\_4&13562&13562&12&11.867&64.031&12&11.867&64.031 \\
lpi\_gosh&13356&3662&9&7.474&5.231&9&27.260&5.231 \\
c-45&13206&13206&5&13.210&85.104&5&13.210&85.104 \\
ca-HepPh&11670&10514&5&20.181&47.173&6&22.400&47.173 \\
coupled&11341&11317&5&8.685&30.083&5&8.704&30.083 \\
c-43&11125&11125&5&11.117&72.602&5&11.117&72.602 \\
psse0&11028&26694&8&9.286&6.075&4&3.836&6.075 \\
psse2&11028&28632&10&10.452&6.713&4&4.026&6.713 \\
c-42&10471&10471&6&10.532&41.339&6&10.532&41.339 \\
nsir&10055&4450&2&15.409&25.894&3&34.817&25.894 \\
c-39&9271&9271&4&14.757&41.233&4&14.757&41.233 \\
wiki-Vote&2355&3728&34&43.018&40.735&8&27.175&40.735 \\
cari&1200&400&1&127.333&178.662&382&382.000&178.662 \\
\end{longtable}
\end{small}

\begin{landscape}
  \section{Result Matrices}
  \label{sec:result_matrices}
  \begin{figure}[b]
    \centering
    \includegraphics[width=.85\linewidth]{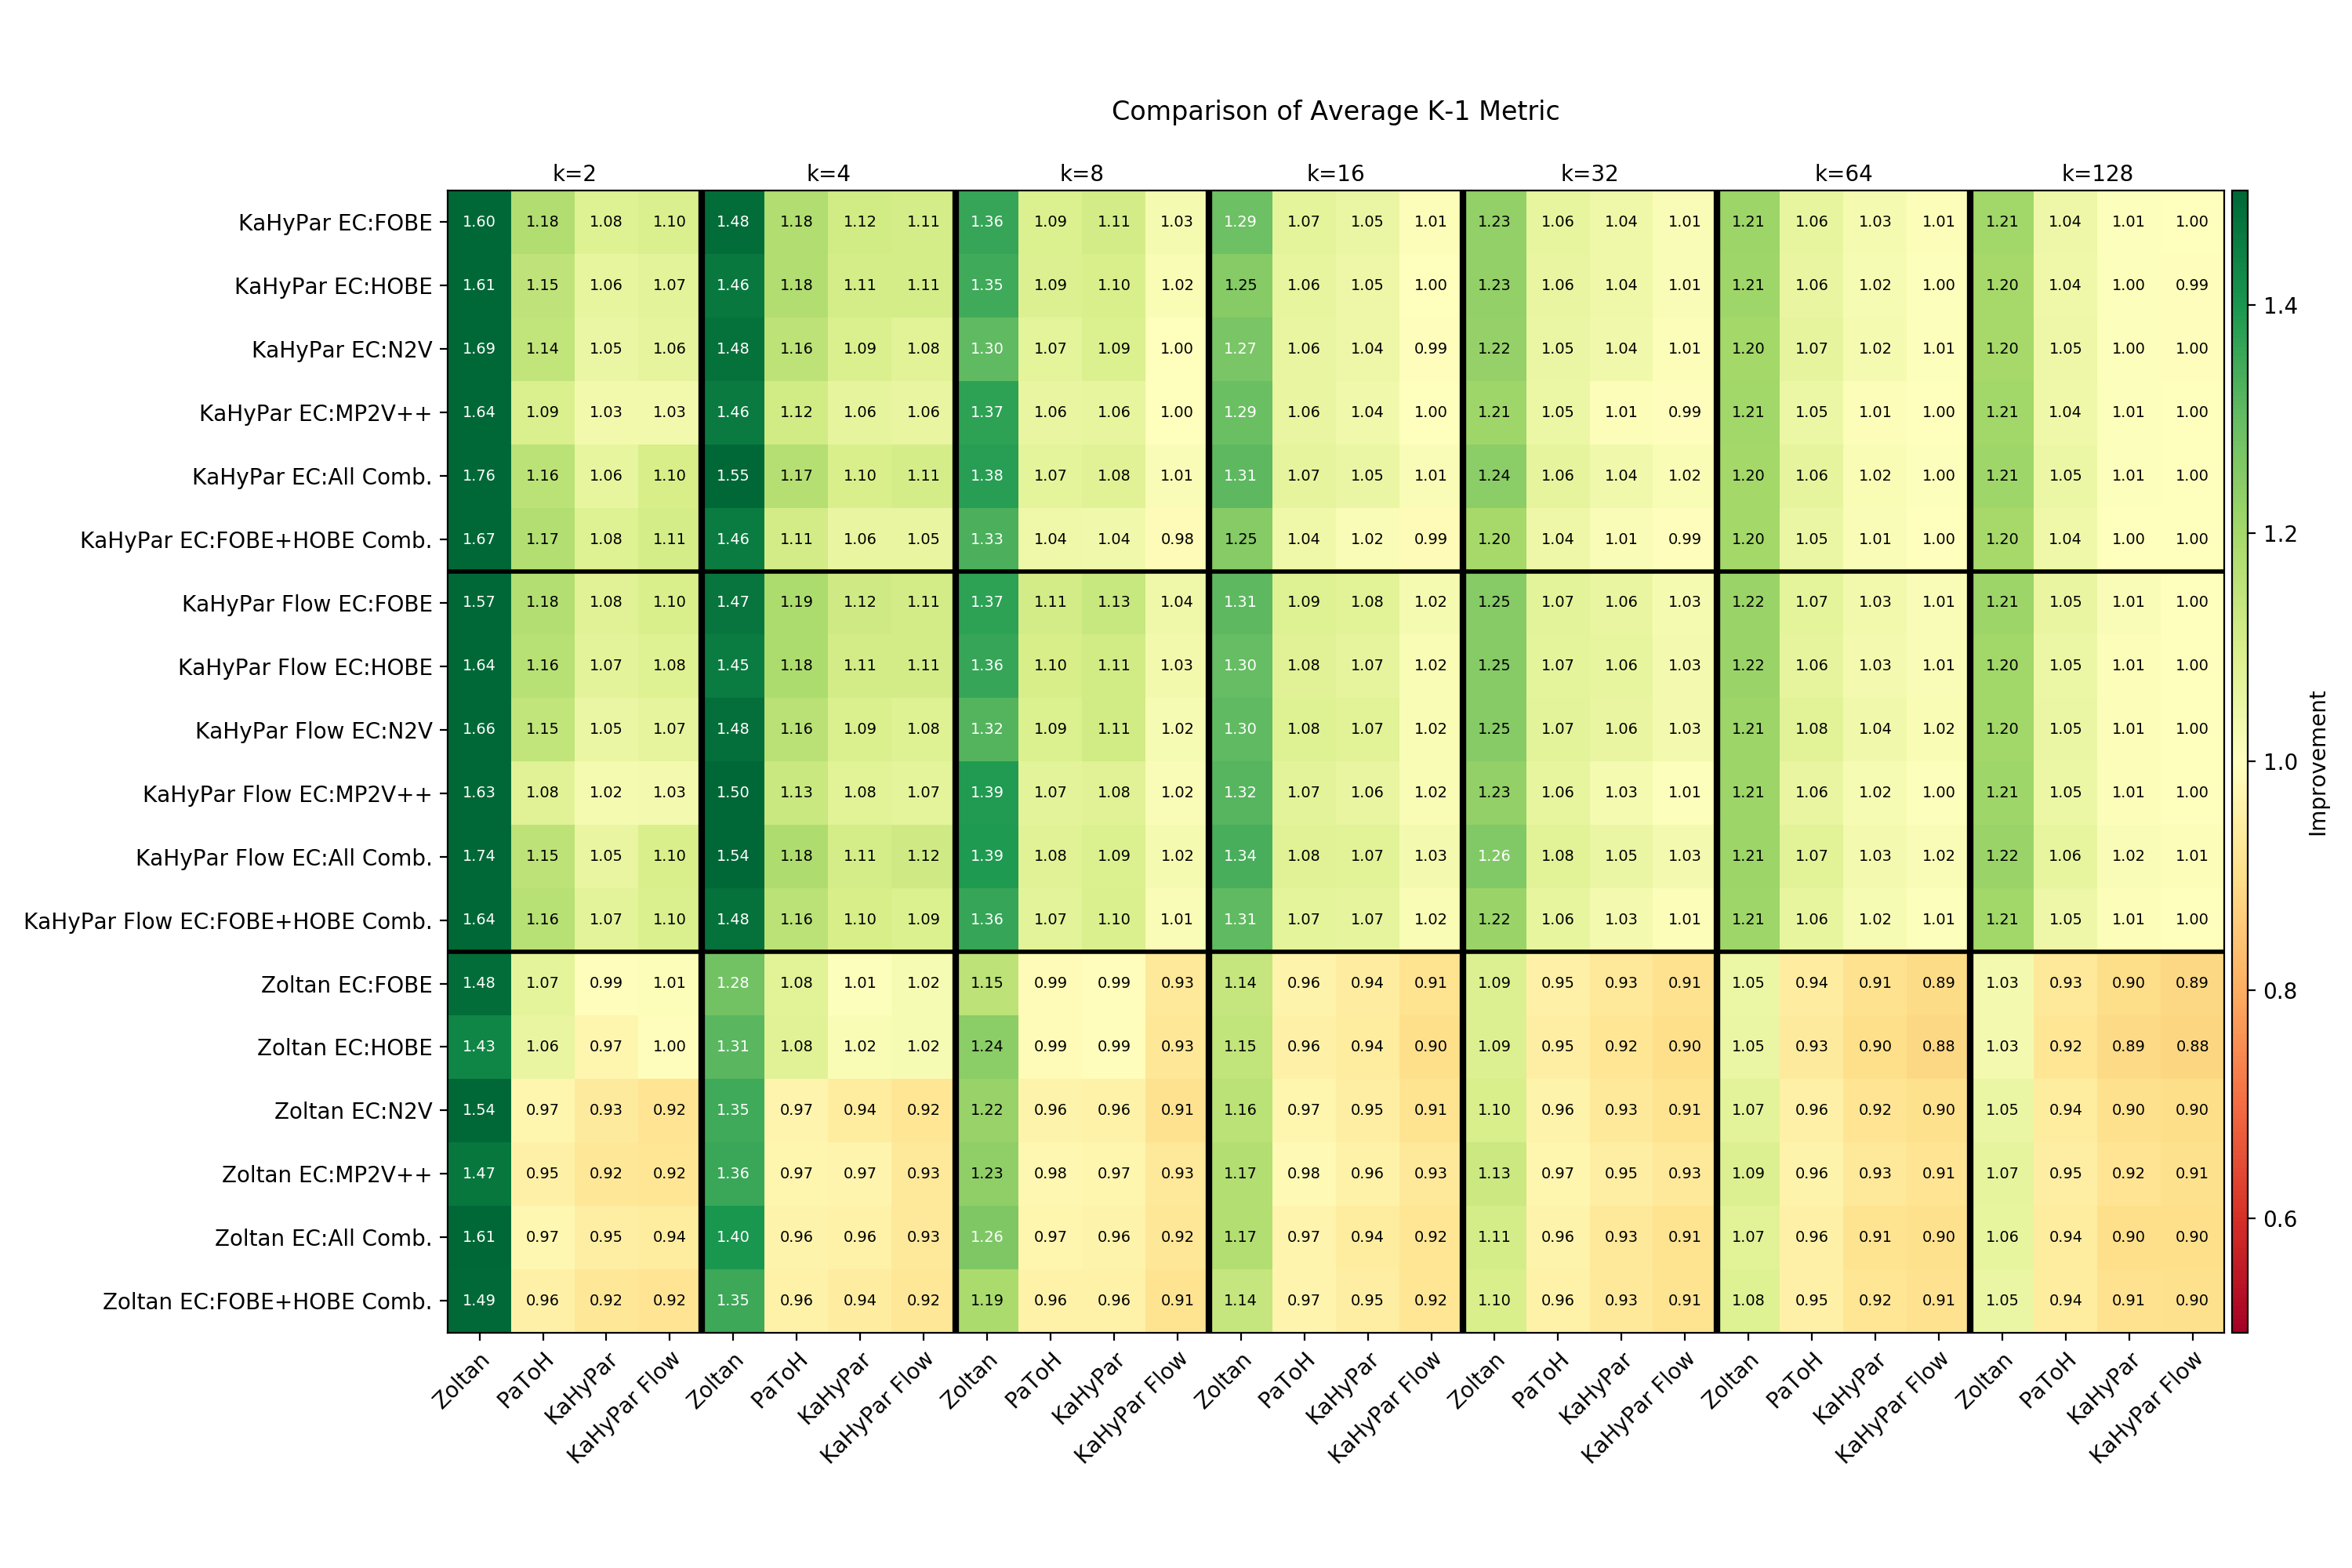}
    \caption{
      Macro-average improvement of the $k-1$ metric across all considered graphs
      and methods.  We performed 20 partitions per-graph per-method using
      different seeds.
    }
    \label{fig:average_km1_matrix}
  \end{figure}
\end{landscape}

\begin{landscape}
  \begin{figure}[p]
      \includegraphics[width=\linewidth]{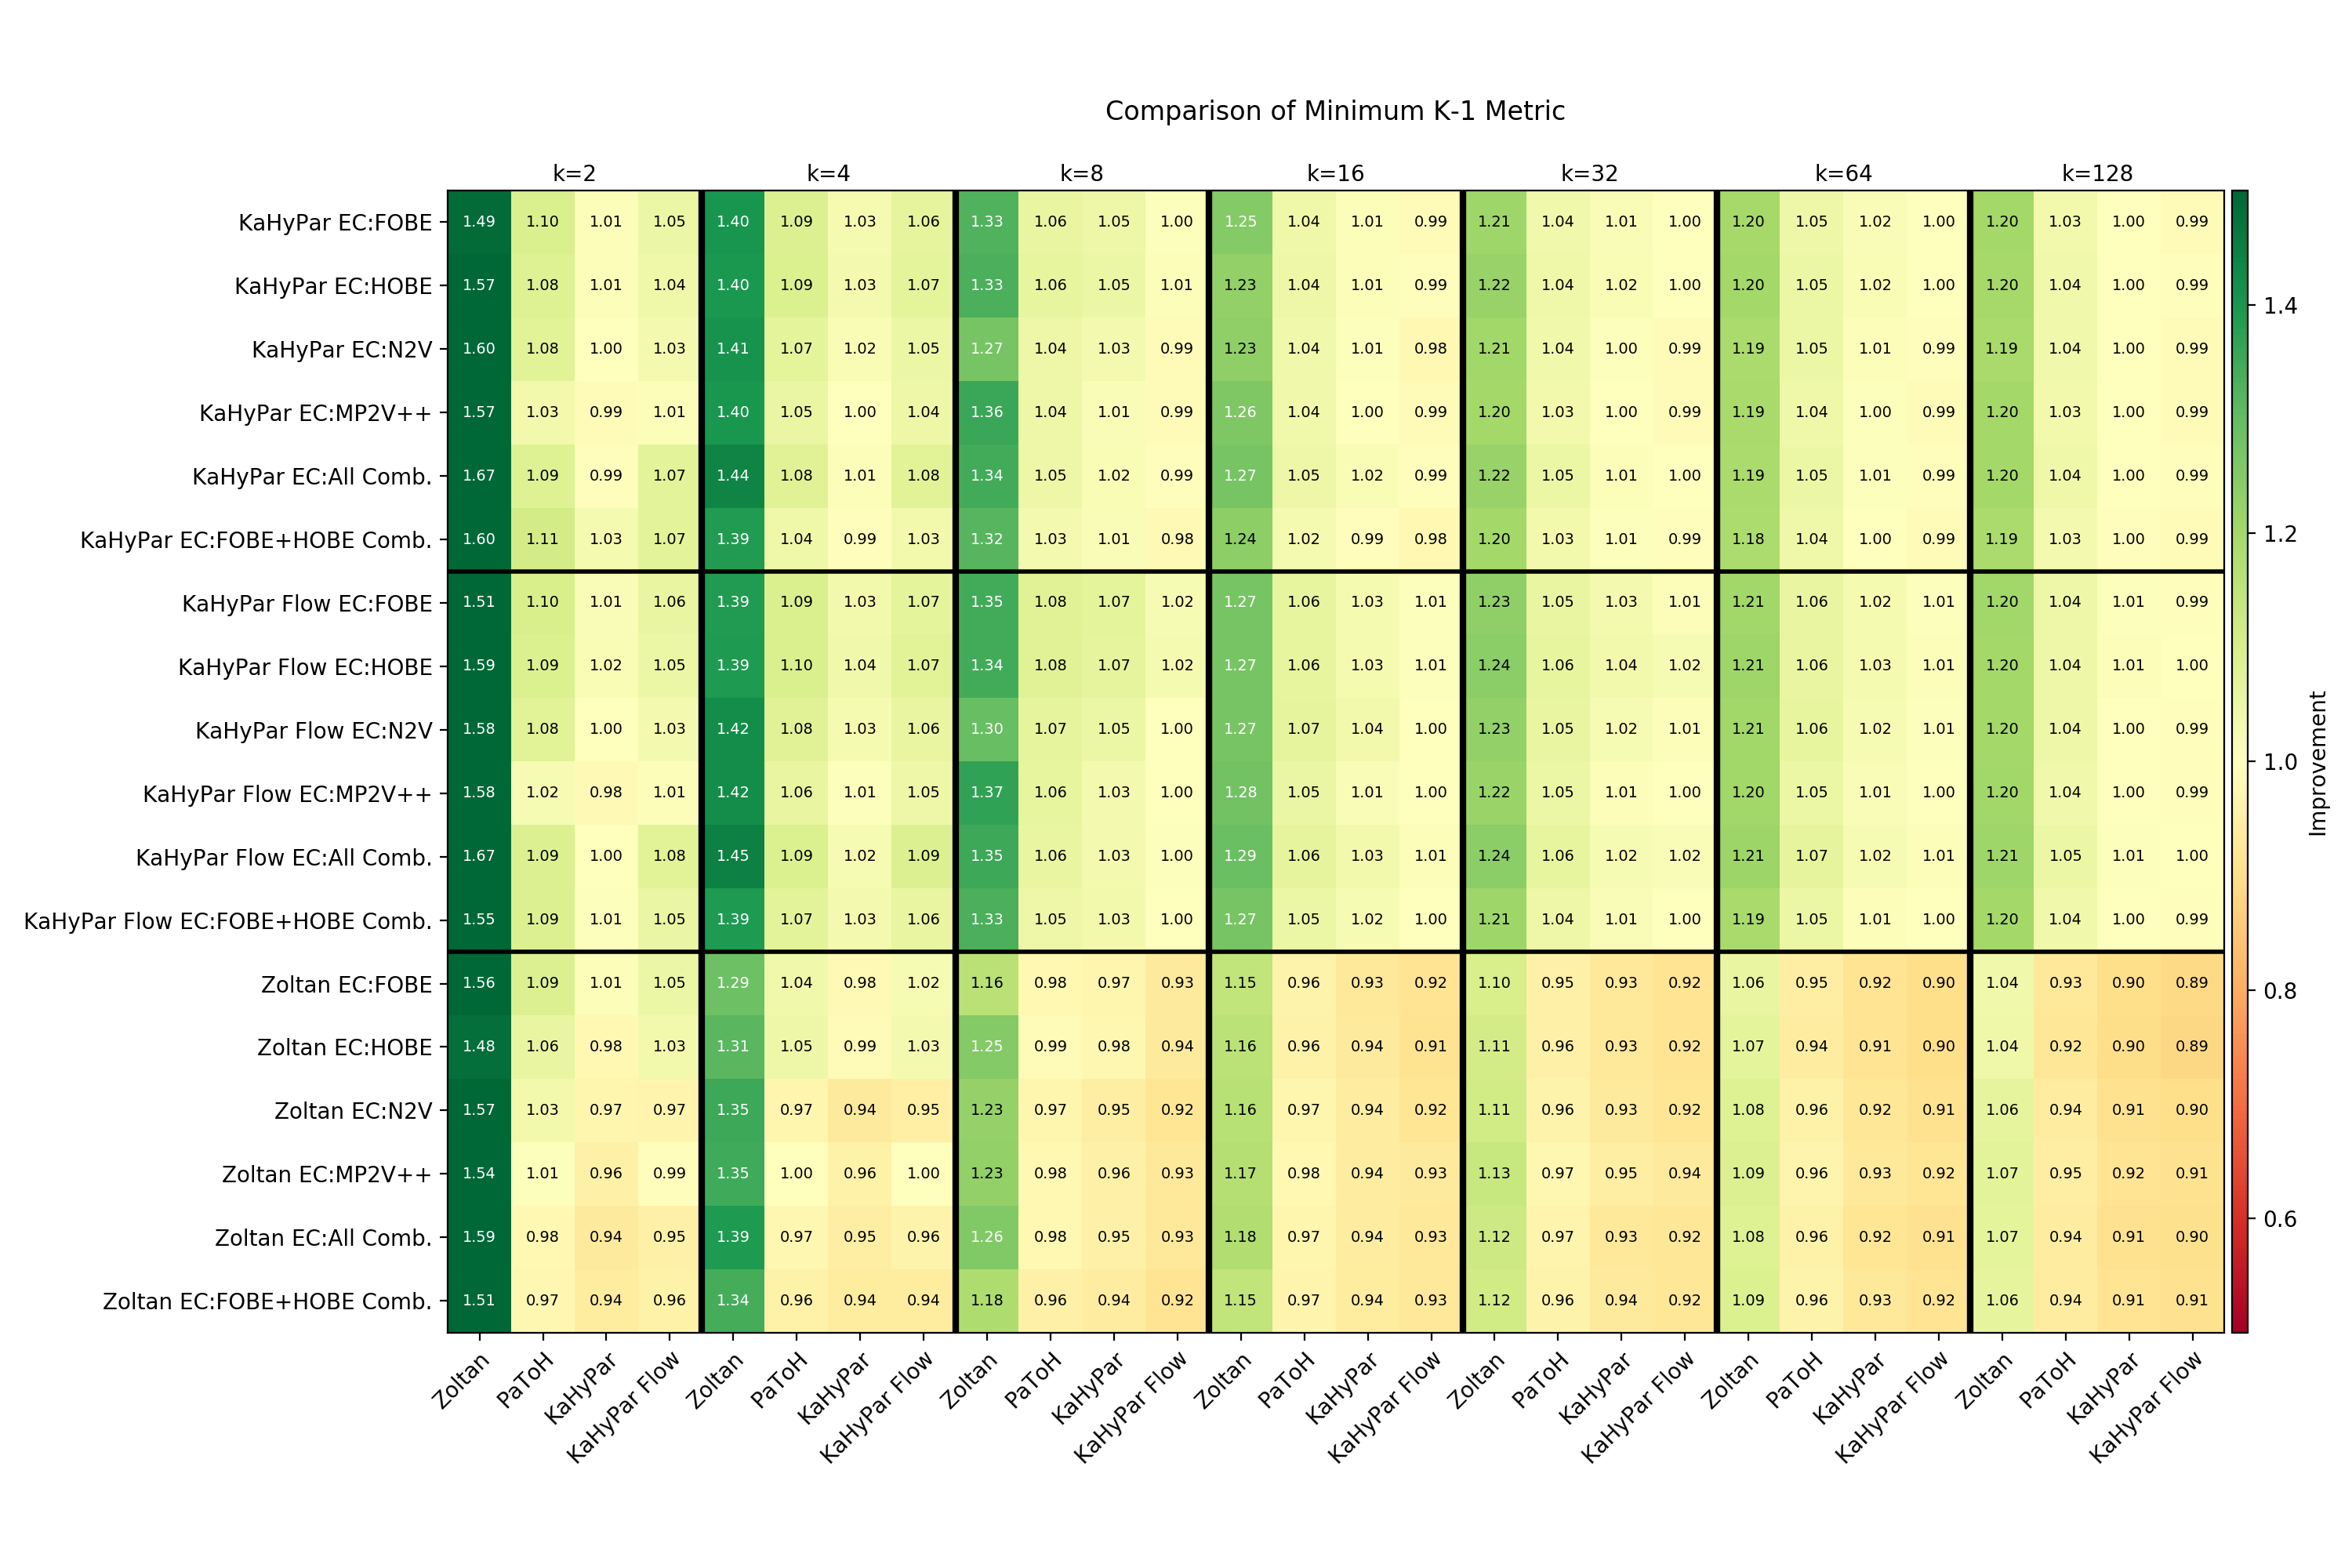}
      \caption{
        Macro-min improvement (ratio of best trails) of the $k-1$ metric across
        all considered graphs.  We performed 20 partitions per-graph per-method
        using different seeds.
      }
      \label{fig:min_km1_matrix}
  \end{figure}
\end{landscape}

\begin{landscape}
  \begin{figure}[p]
      \includegraphics[width=\linewidth]{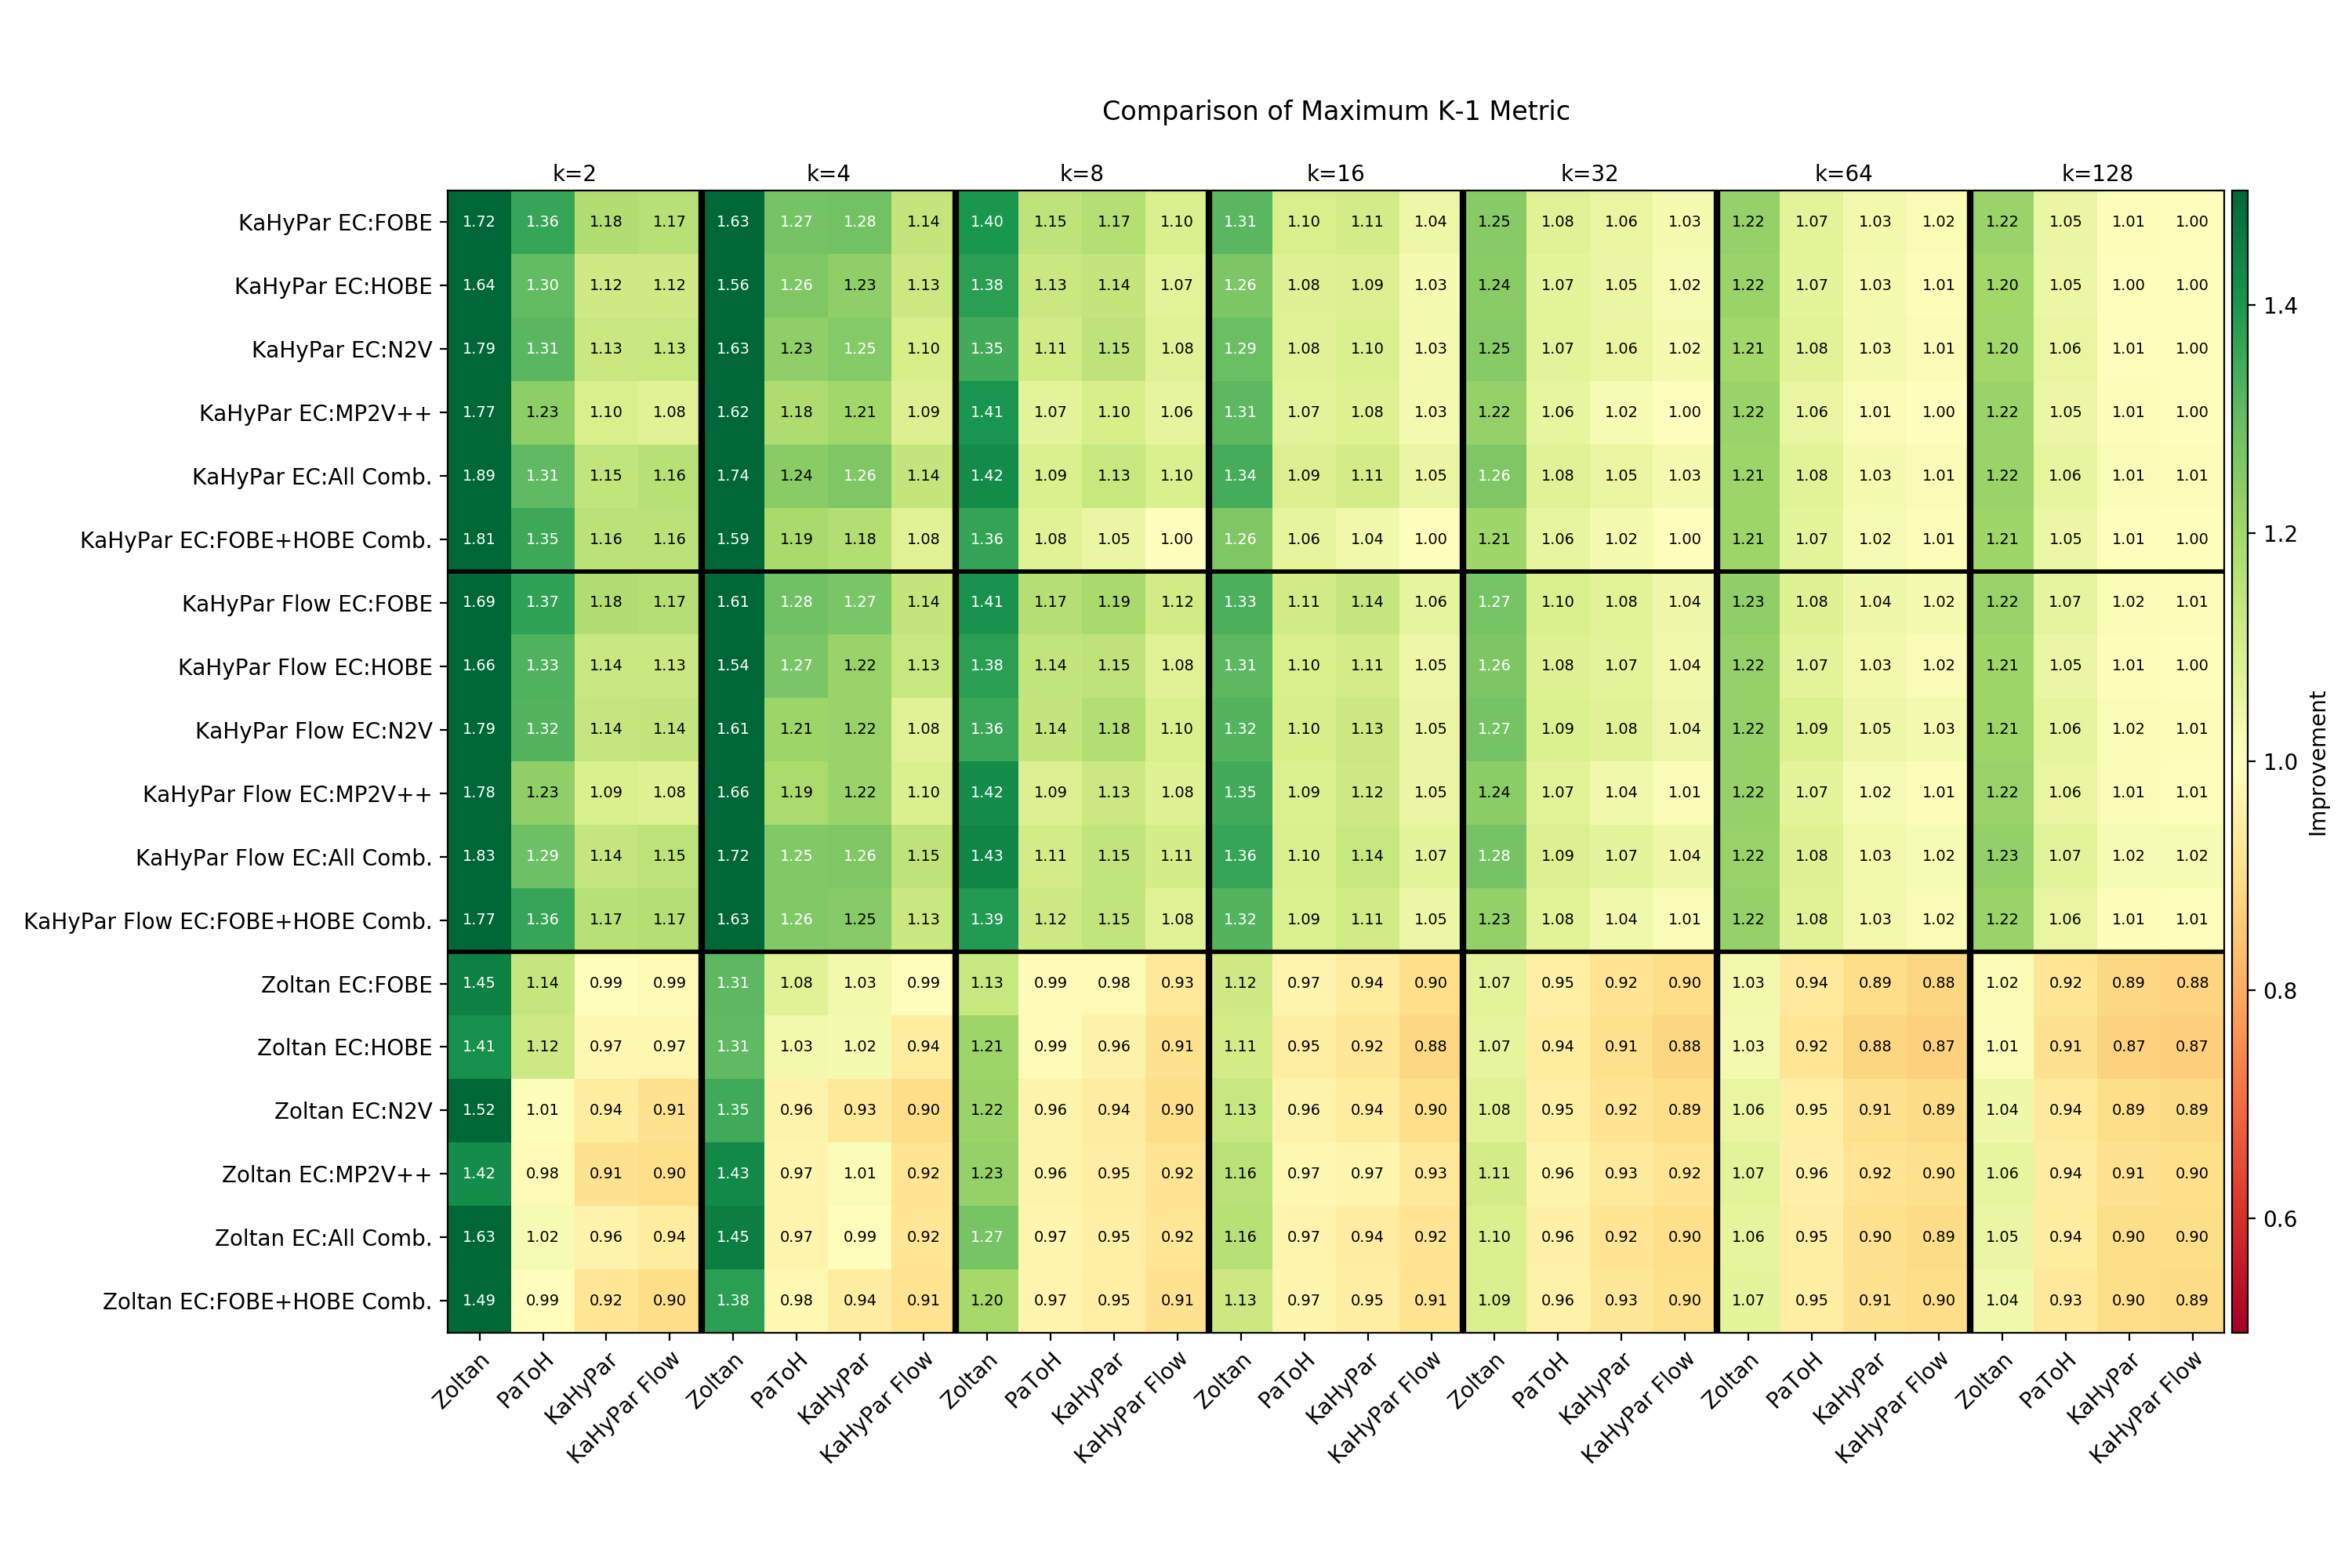}
      \caption{
        Macro-max improvement (ratio of worst trails) of the $k-1$ metric across
        all considered graphs.  We performed 20 partitions per-graph per-method
        using different seeds.
      }
      \label{fig:max_km1_matrix}
  \end{figure}
\end{landscape}

\begin{landscape}
  \begin{figure}[p]
      \includegraphics[width=\linewidth]{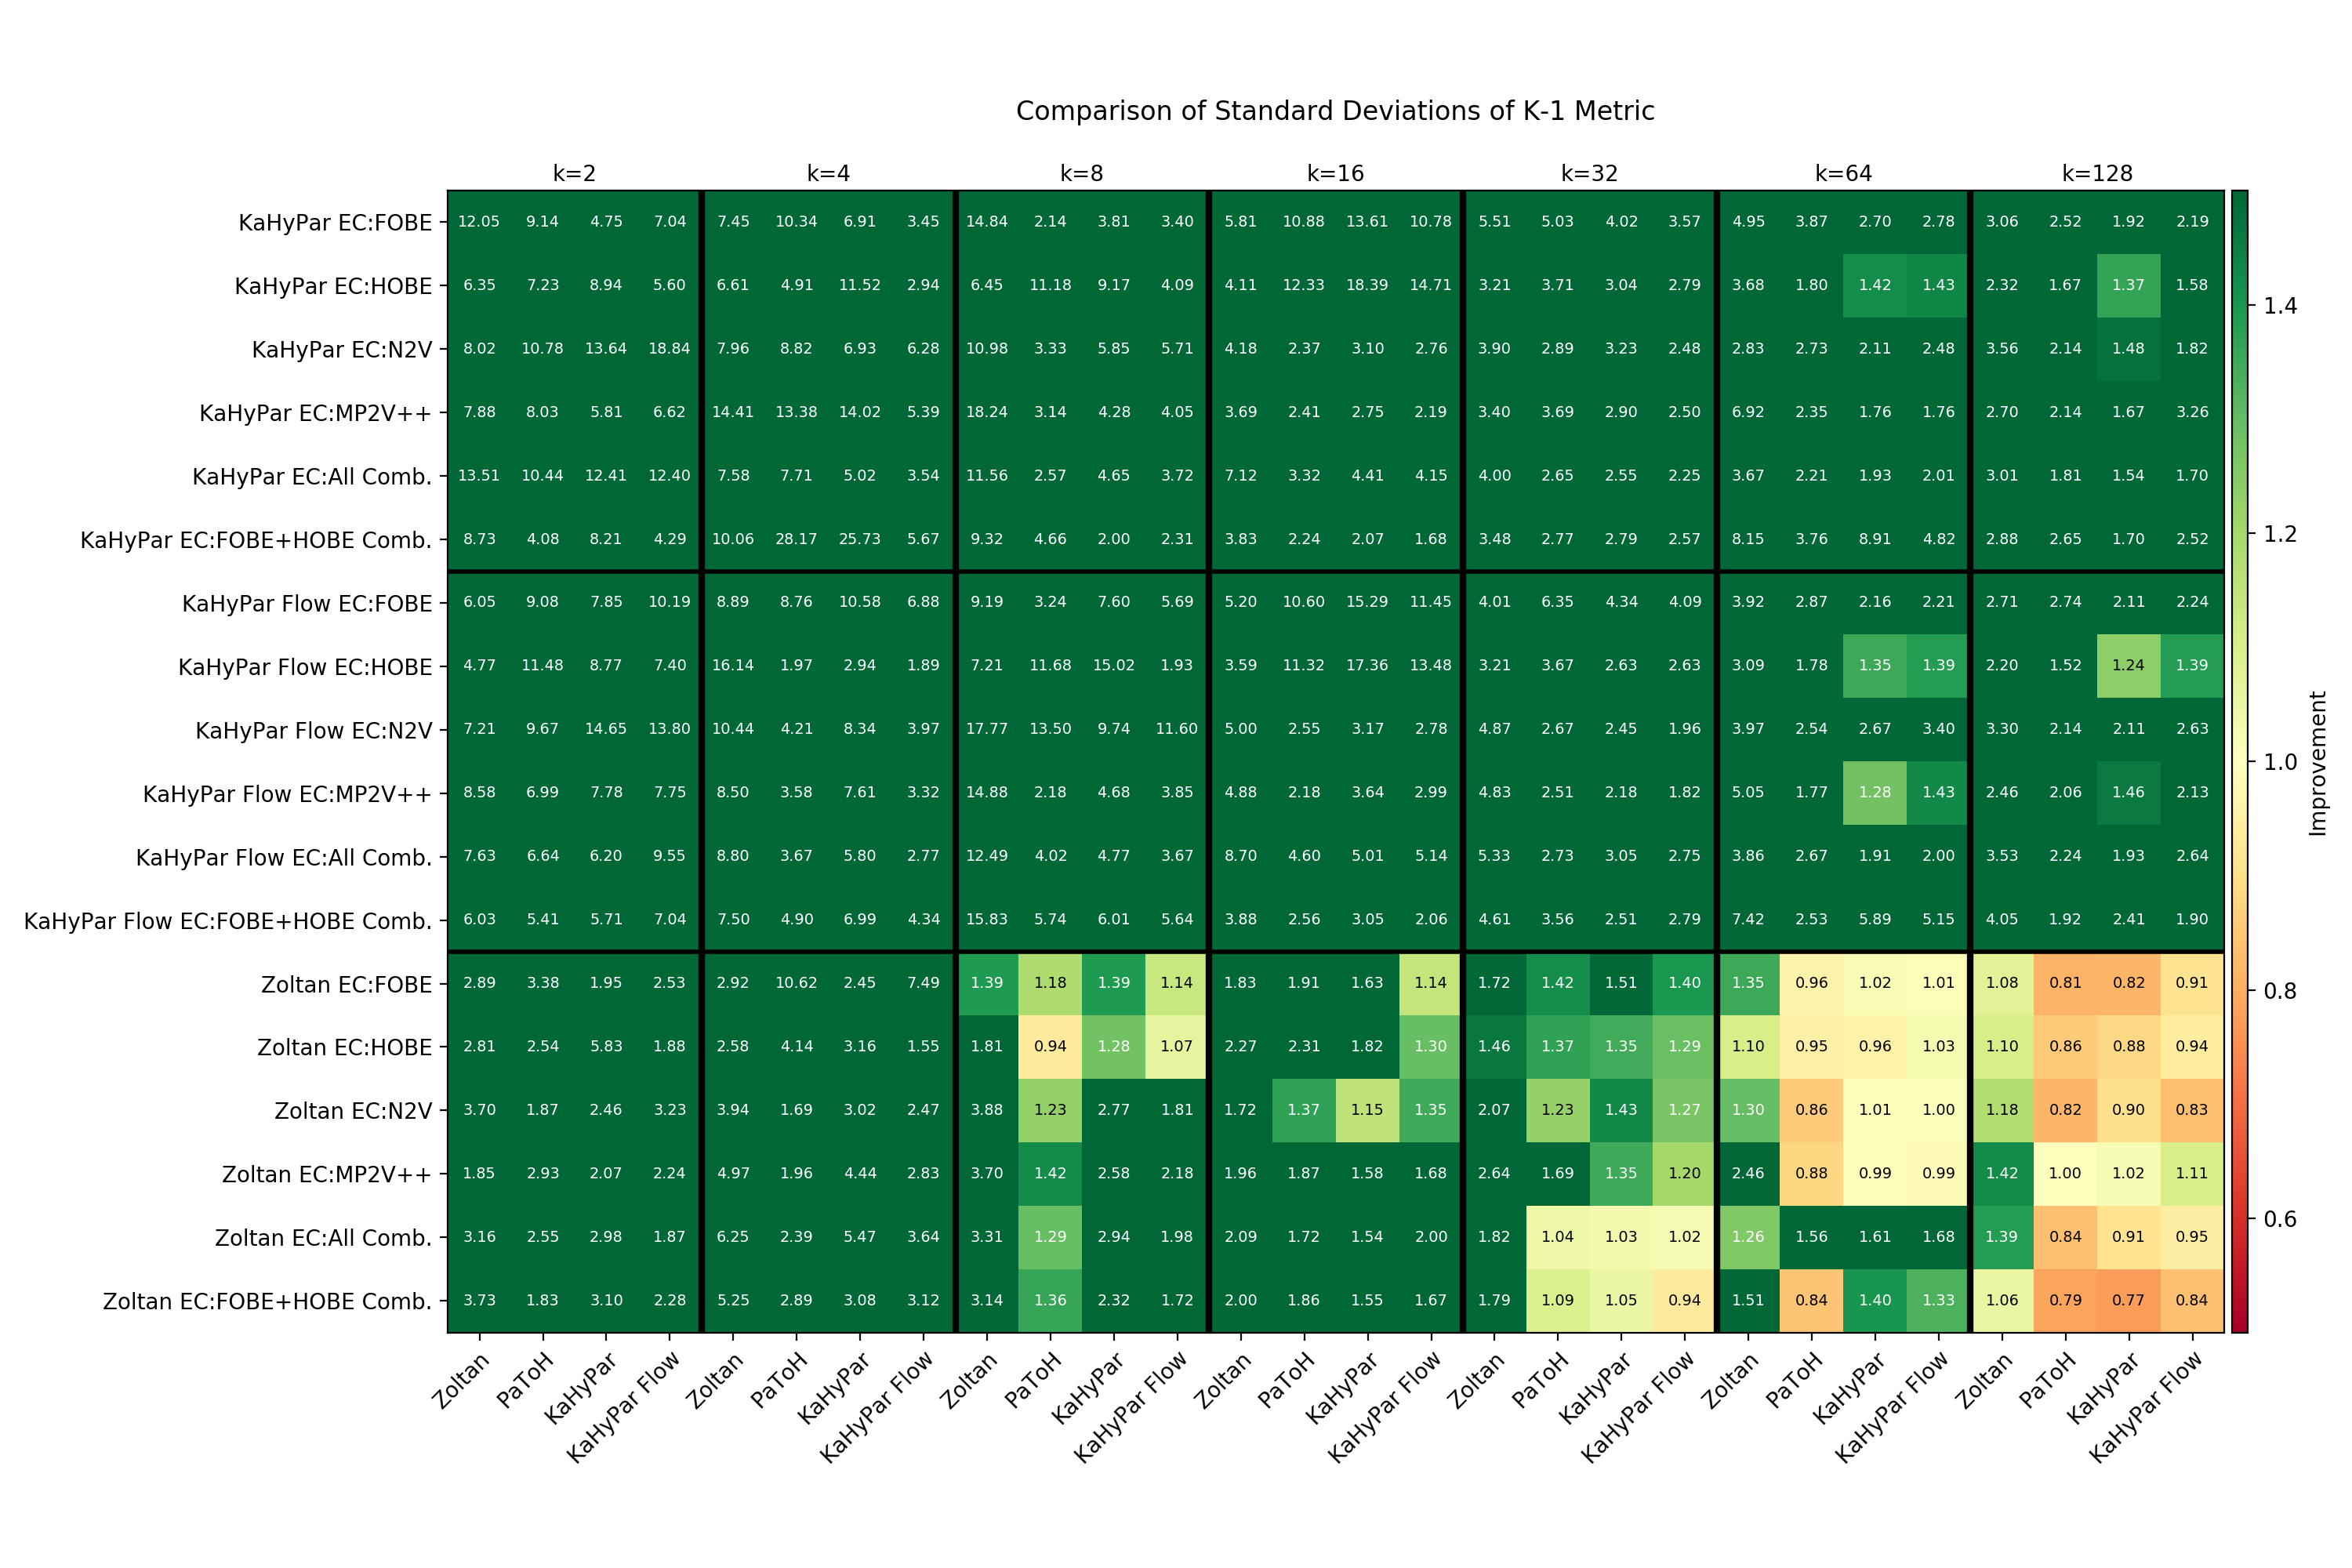}
      \caption{
        Average improvement of the standard deviation of the $k-1$ metric across
        all considered graphs. We performed 20 partitions per-graph per-method
        using different seeds.
      }
      \label{fig:std_km1_matrix}
  \end{figure}
\end{landscape}

\begin{landscape}
  \begin{figure}[p]
      \includegraphics[width=\linewidth]{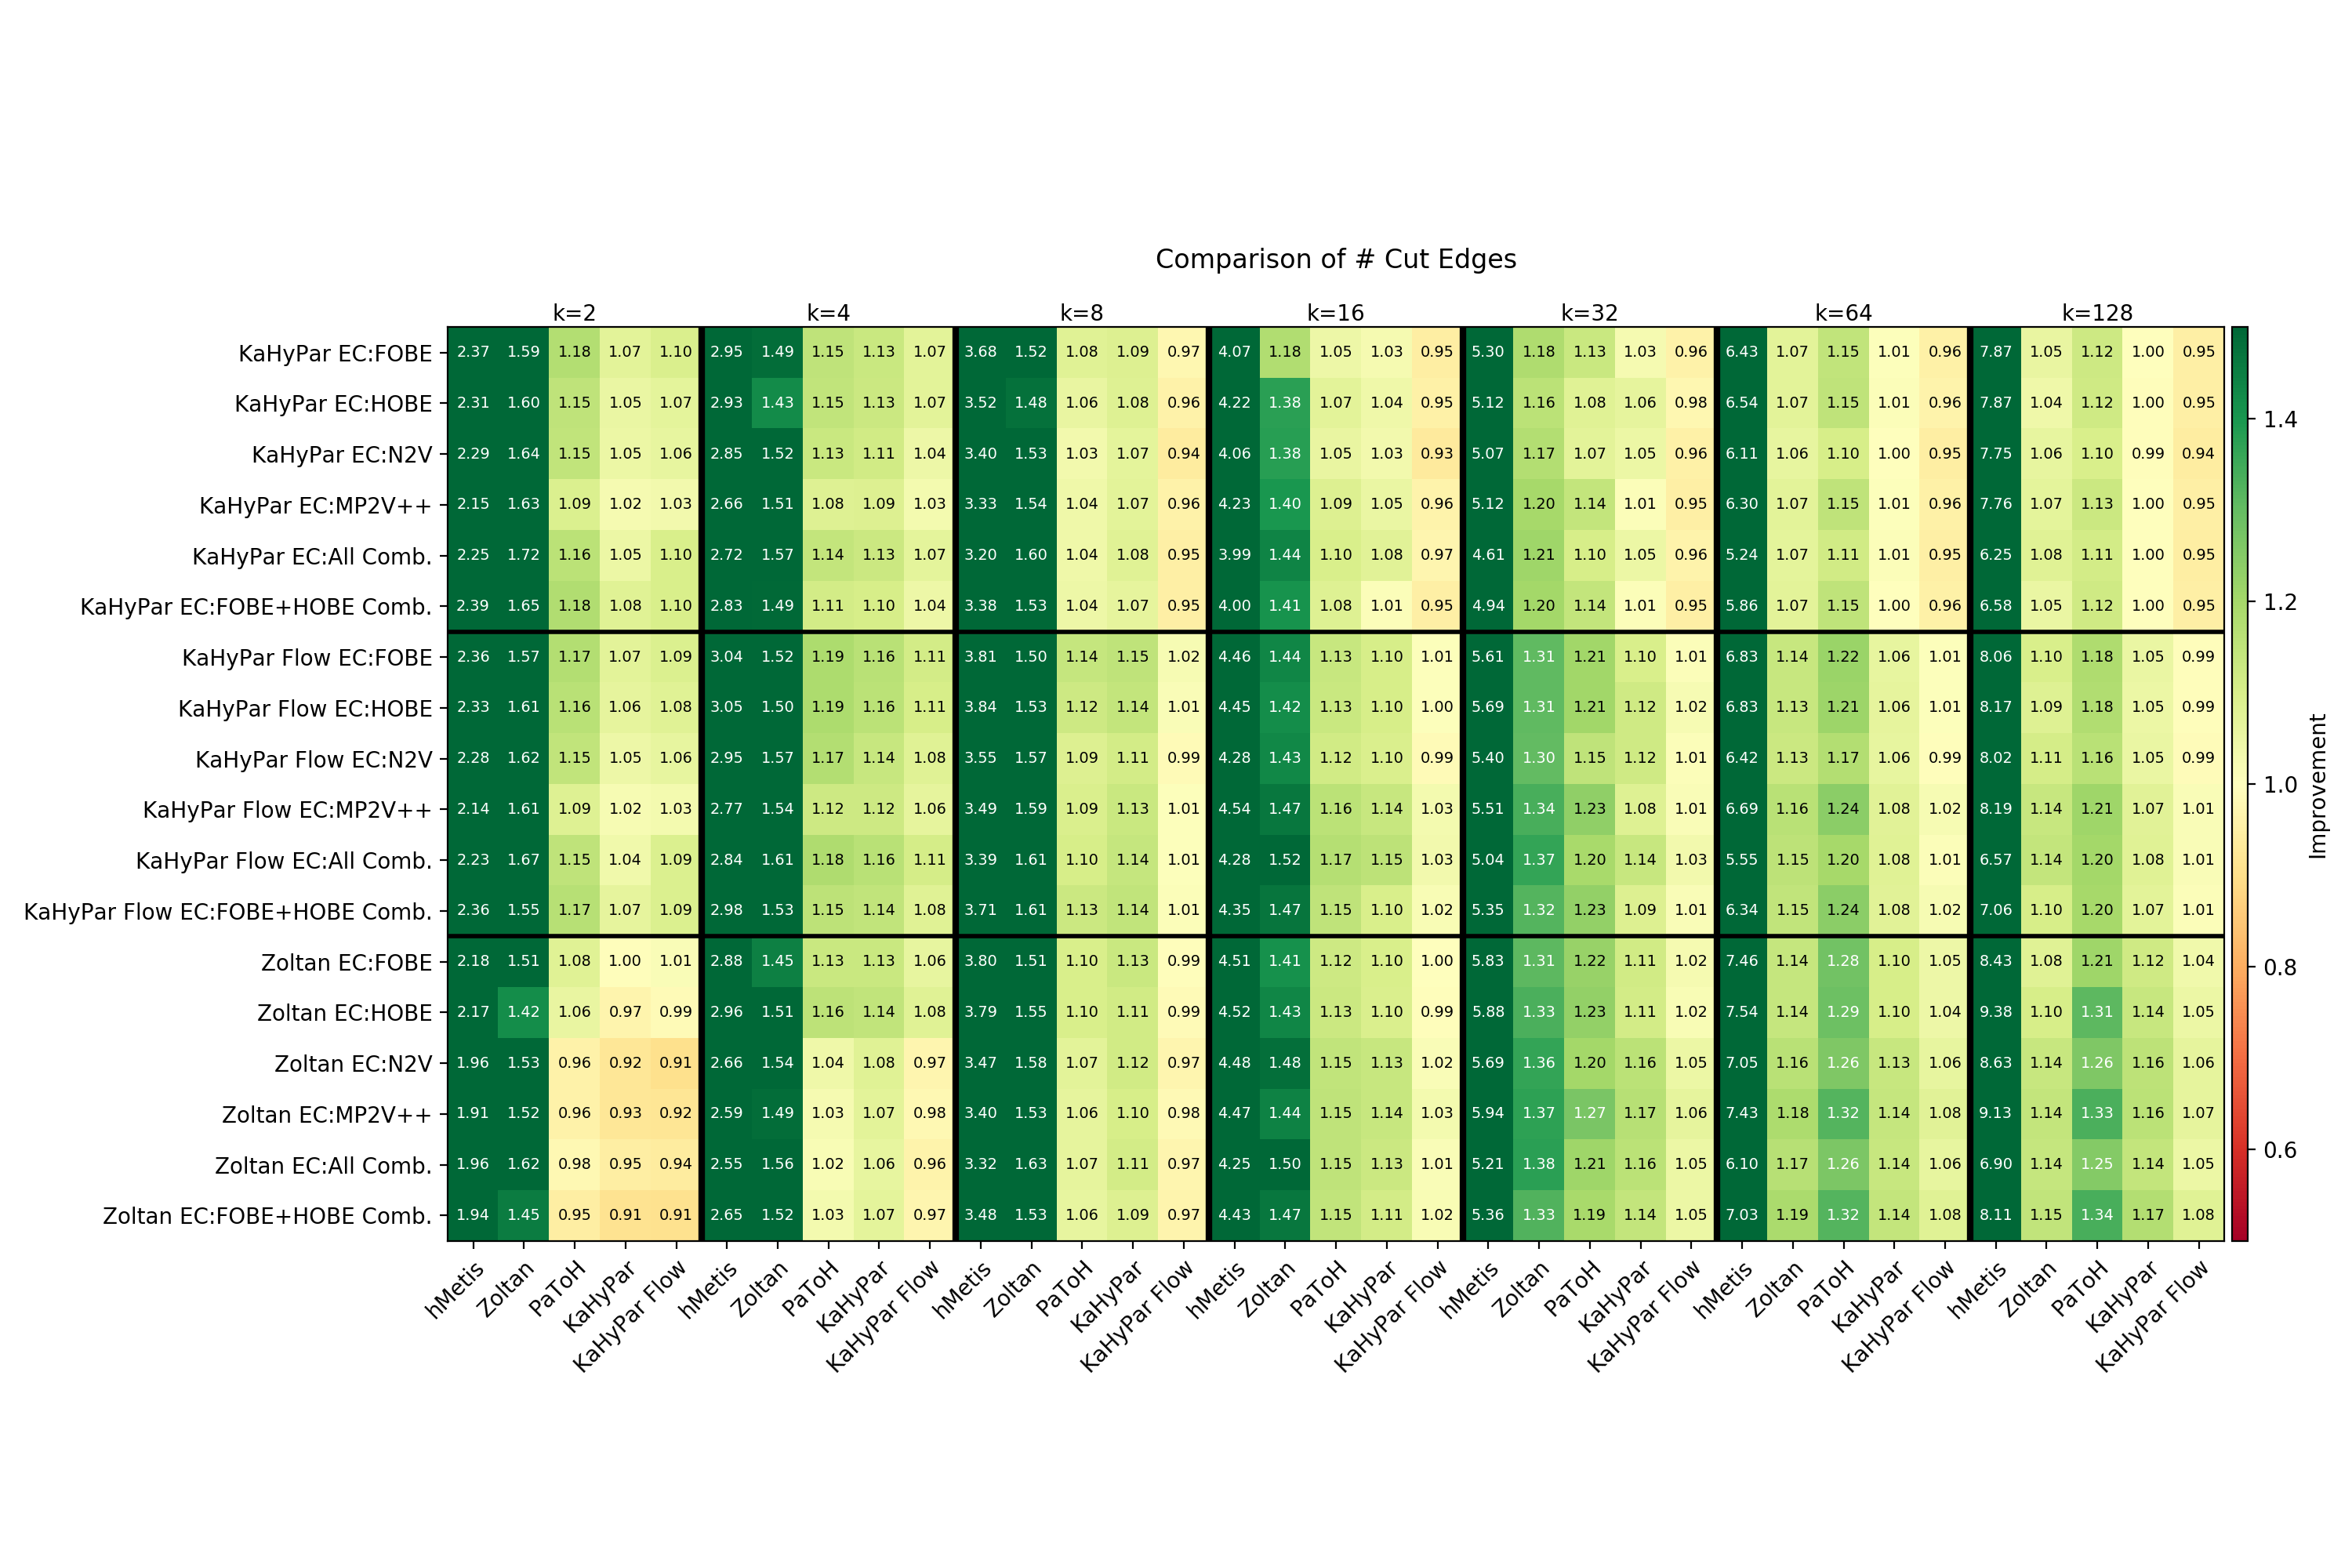}
      \caption{
        Macro-average improvement of the \# cut hyperedges metric across all
        considered graphs and methods.  We performed 20 partitions per-graph
        per-method using different seeds.
      }
      \label{fig:average_cut_matrix}
  \end{figure}
\end{landscape}

\begin{landscape}
  \begin{figure}[p]
      \includegraphics[width=\linewidth]{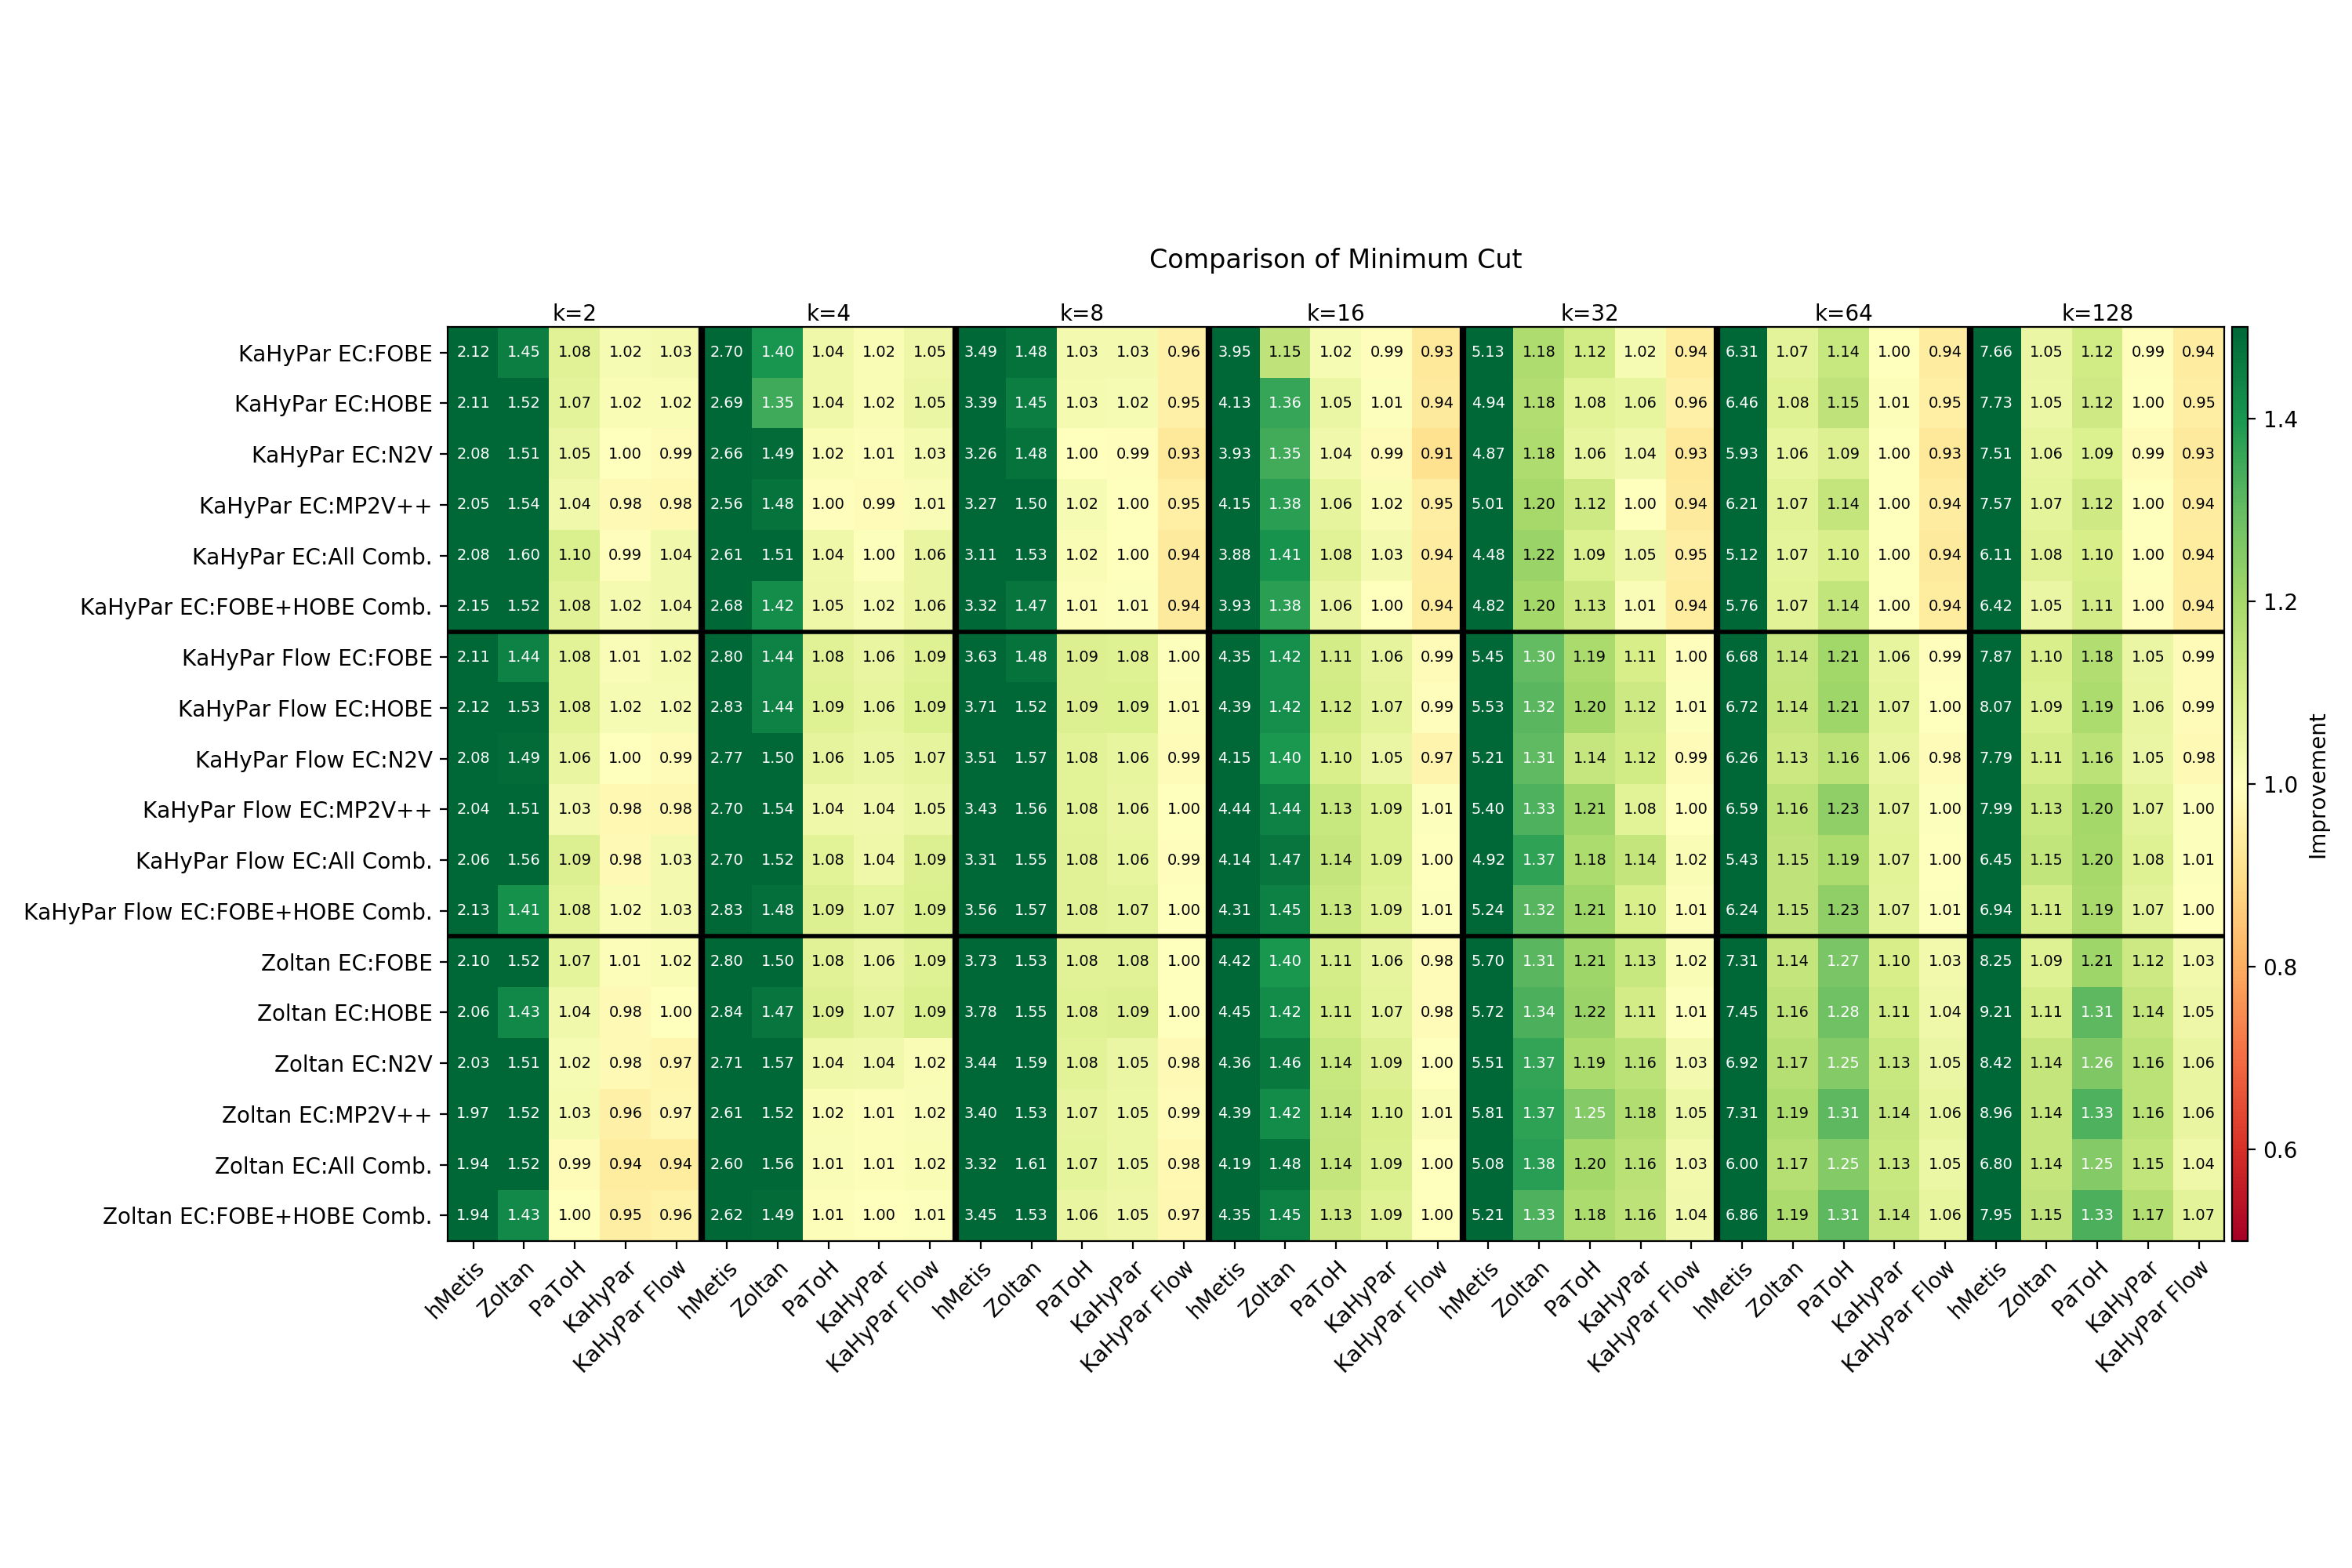}
      \caption{
        Macro-min improvement (ratio of best trails) of the \# cut hyperedges
        metric across all considered graphs.  We performed 20 partitions
        per-graph per-method using different seeds.
      }
      \label{fig:min_cut_matrix}
  \end{figure}
\end{landscape}

\begin{landscape}
  \begin{figure}[p]
      \includegraphics[width=\linewidth]{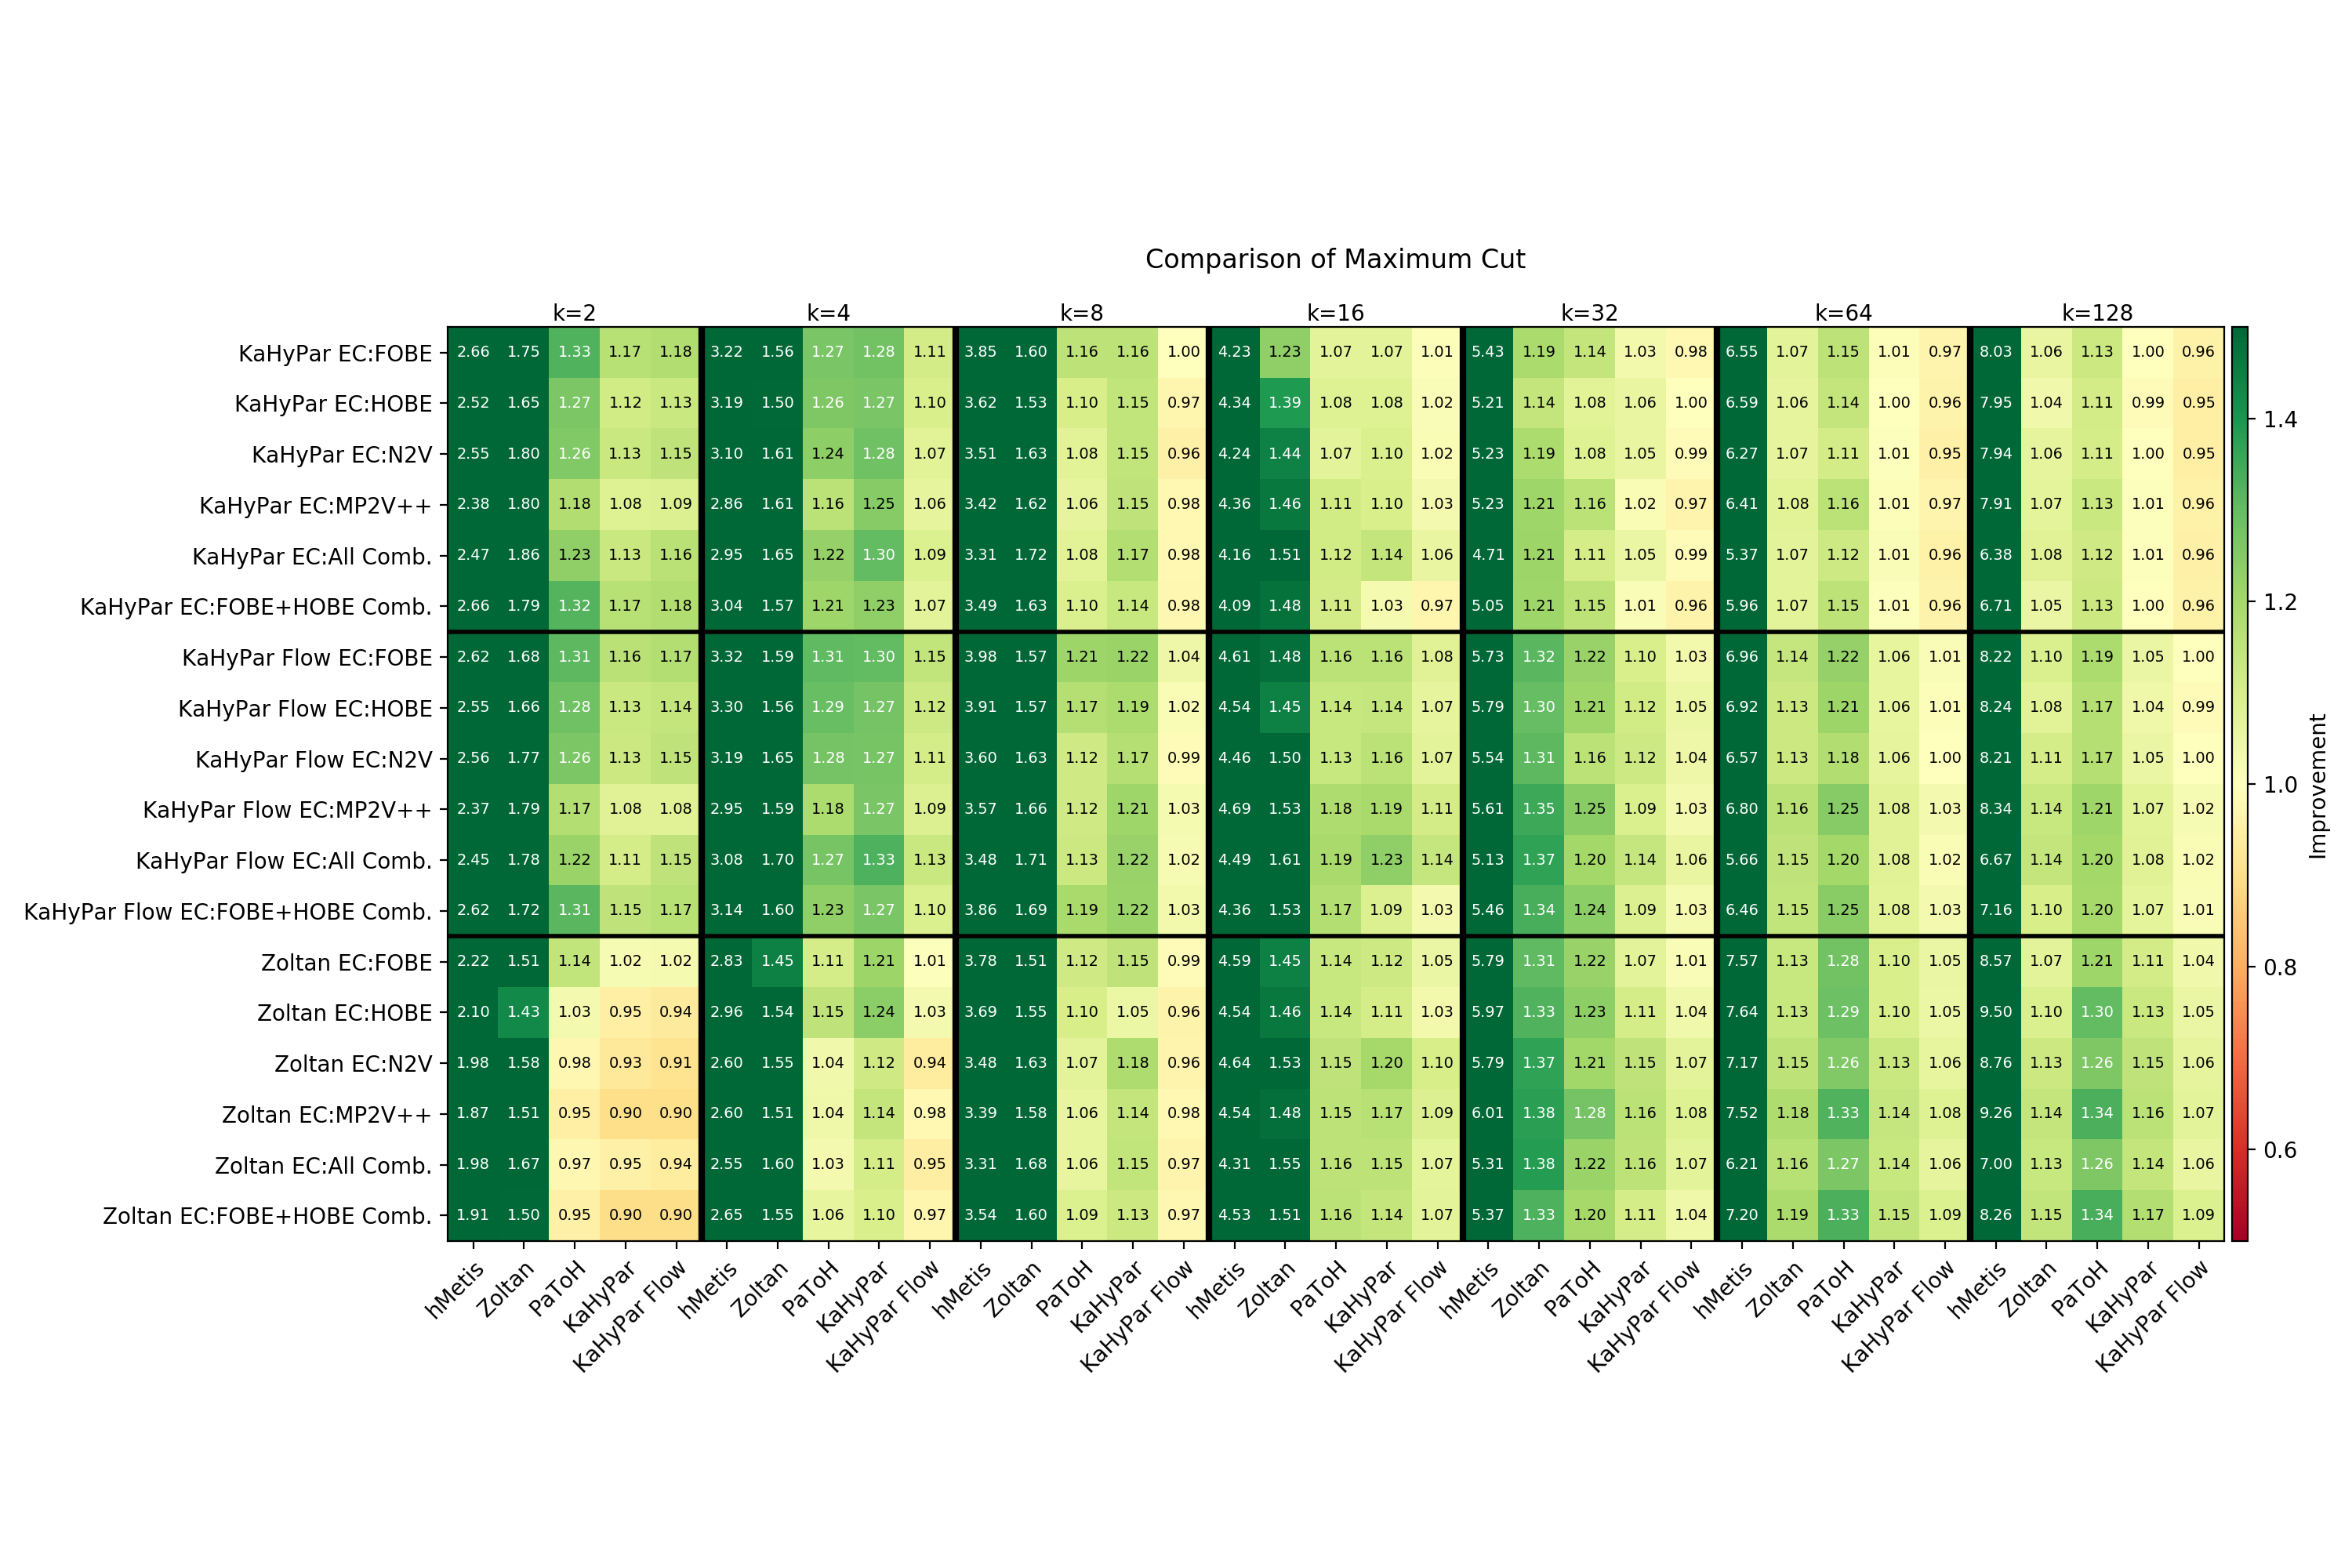}
      \caption{
        Macro-max improvement (ratio of worst trails) of the \# cut hyperedges
        metric across all considered graphs.  We performed 20 partitions
        per-graph per-method using different seeds.
      }
      \label{fig:max_cut_matrix}
  \end{figure}
\end{landscape}

\begin{landscape}
  \begin{figure}[p]
      \includegraphics[width=\linewidth]{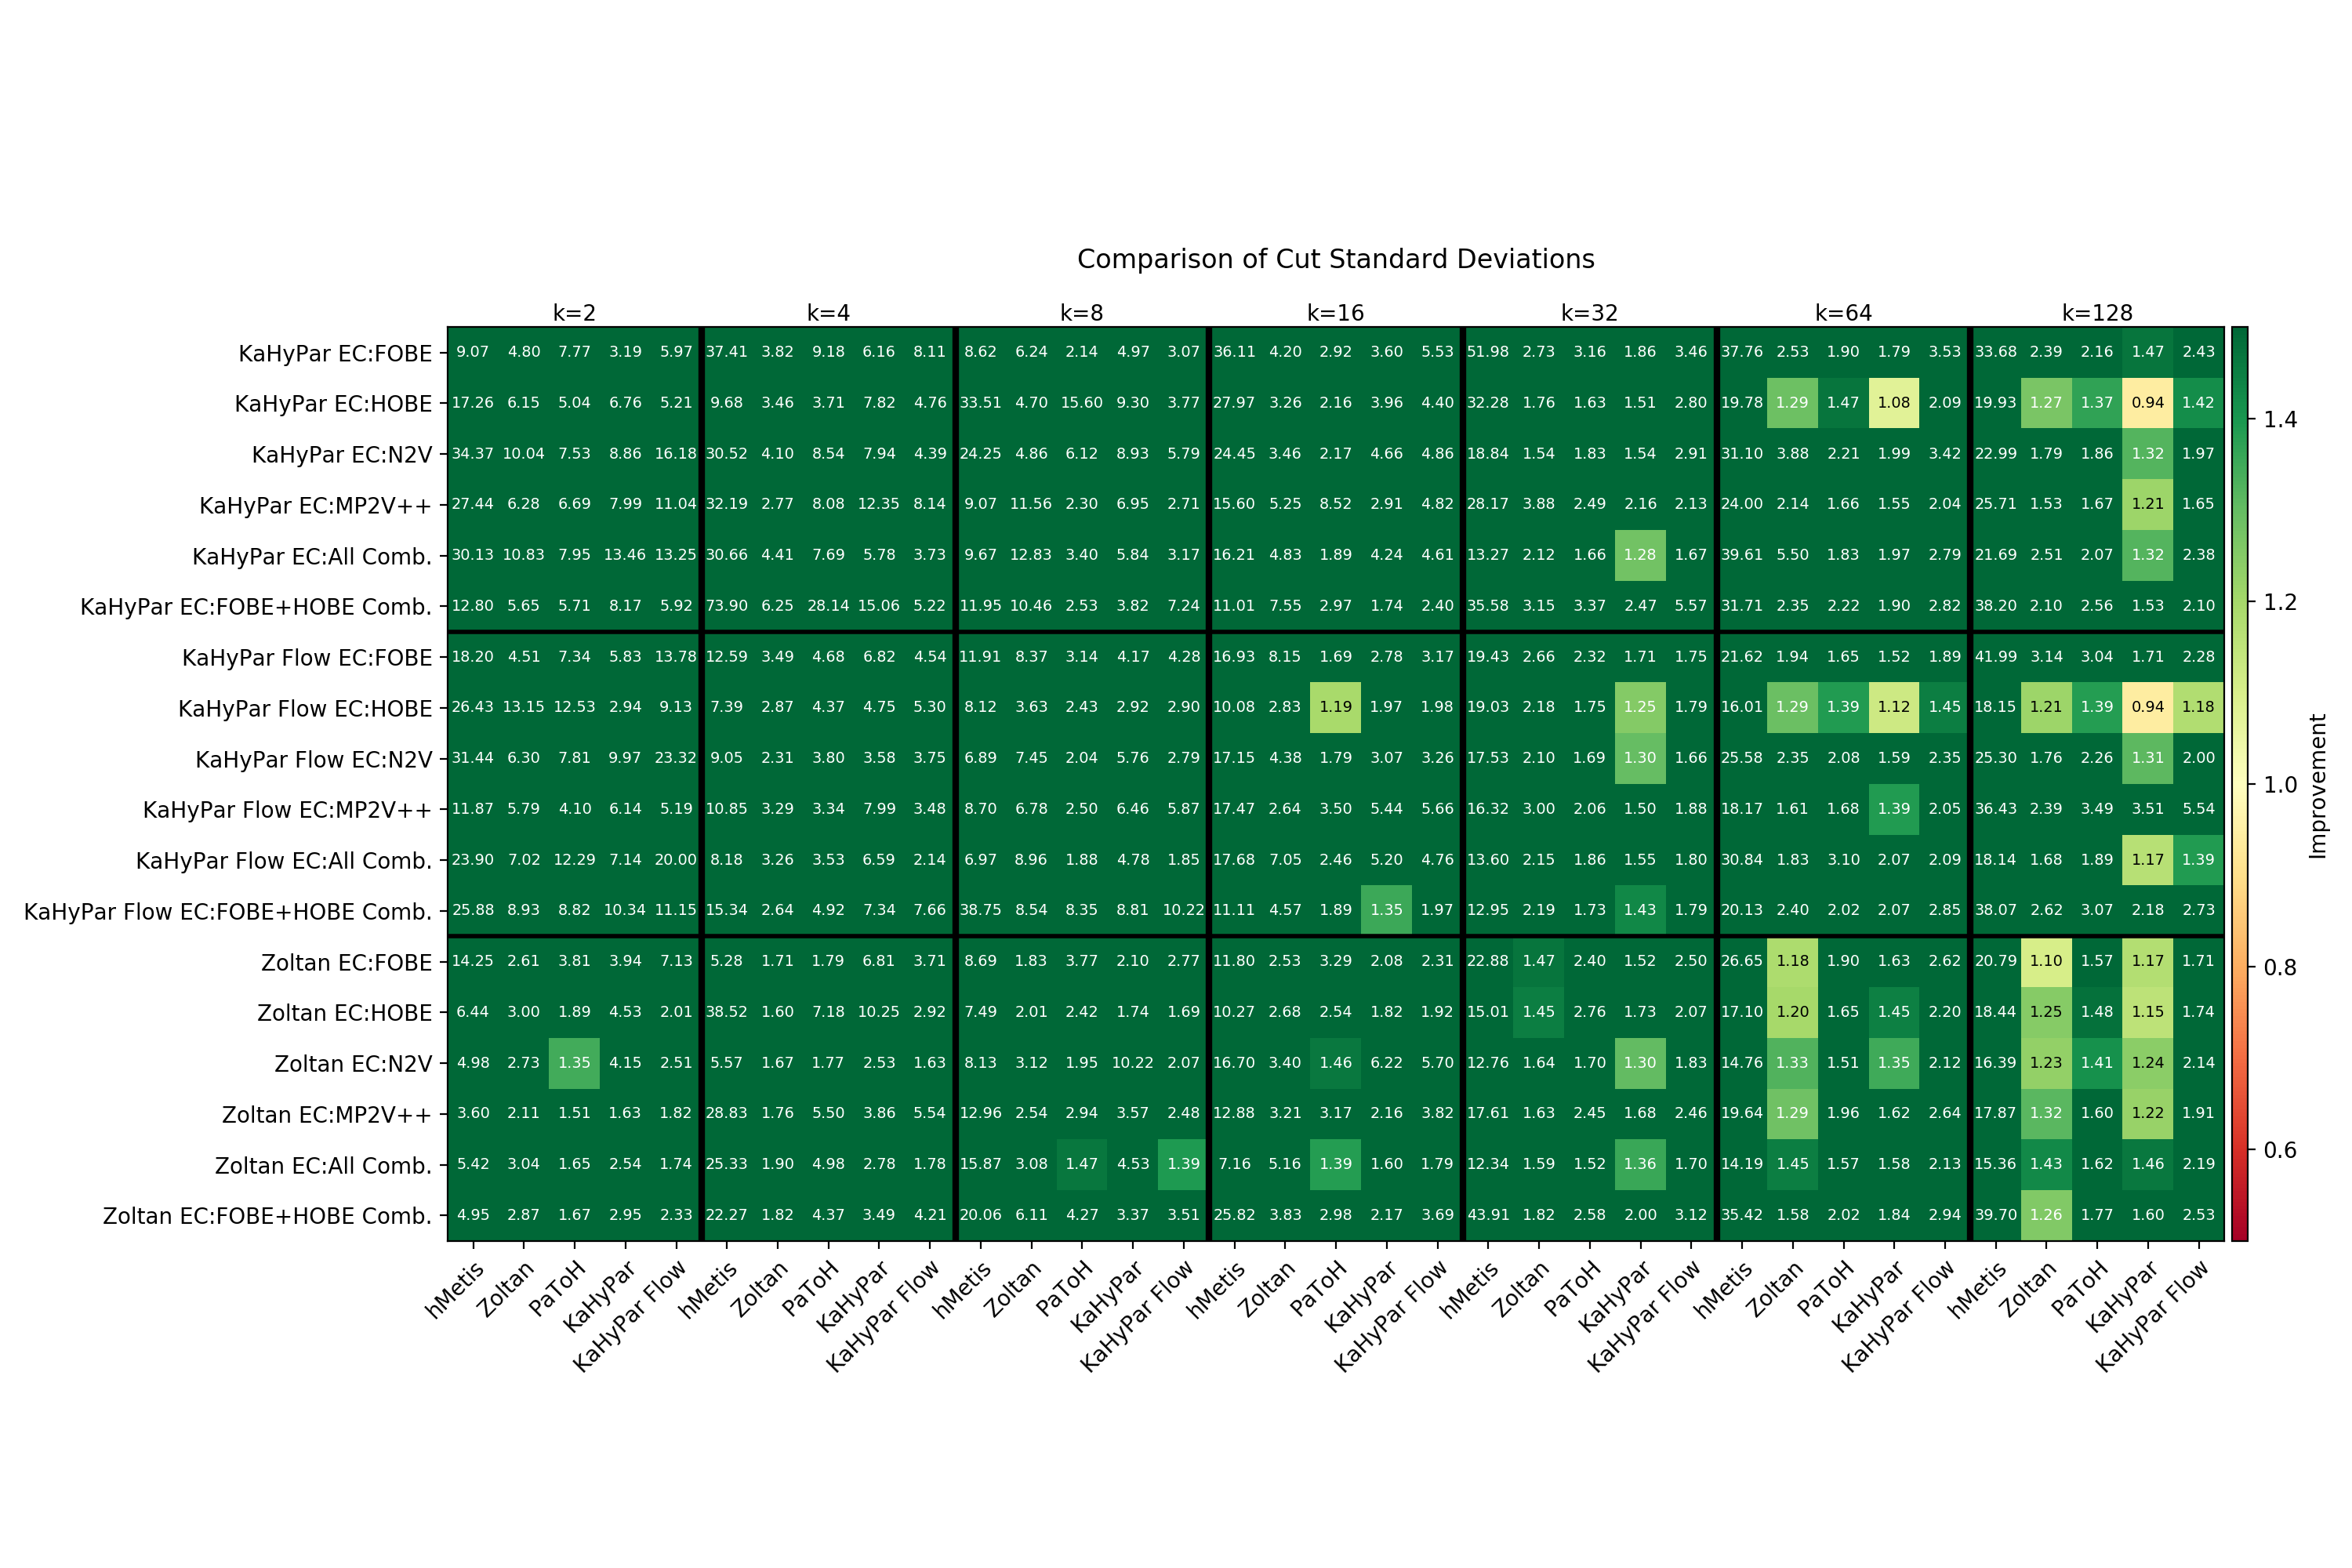}
      \caption{
        Average improvement of the standard deviation of the \# cut hyperedges
        metric across all considered graphs. We performed 20 partitions
        per-graph per-method using different seeds.
      }
      \label{fig:std_cut_matrix}
  \end{figure}
\end{landscape}
